# Supplementary material for: Effect of perturbations on the kagome $S=1/2$ antiferromagnet at all temperatures
Source: arXiv:1909.00993 ancillary file (2020-01-06)
Supplement: Supplementary file 1 [file KagJ1_Detailed.pdf]

# Specific heat and magnetic susceptibility of the spin-1/2 Heisenberg model on kagome lattice


Bernard Bernu,[1] Laurent Pierre,[2] Karim Essafi,[1] and Laura Messio[1,3]

[1] *Sorbonne Université, CNRS, Laboratoire de Physique Théorique de la Matière Condensée, LPTMC, F-75005 Paris, France*[*]
[2] *Paris X, Nanterre*
[3] *Institut Universitaire de France (IUF), F-75005 Paris, France*[†]



(Dated: January 6, 2020)



This supplemental material gives some details on the results obtained on the specific heat, $C_V(T)$, and the magnetic susceptibility, $\mathcal{X}(T)$, of the antiferromagnetic Heisenberg model on the kagome lattice, using high temperature series expansions (HTSE) and an extrapolating scheme assuming $S = 1/2$-non gapped as well as gapped low temperature physics, named the entropy method and denoted HTSE+$s(e)$. Various perturbations are explored: impurities, magnetic field, Dzyaloshinskii–Moriya interaction, Ising interaction, second and third neighbor interactions. For all the models used here, new HTSE have been calculated or a few more terms have been added to existing series. Convergence is studied in detail through curves for the raw series in $\beta = 1/T$ and their Padé approximants (PAs), of the raw series in the energy $e$ (obtained from a Legendre transformation of the previous ones) and their PAs, and of the HTSE+$s(e)$ results. Methods to self-consistently extract the necessary input parameters of the HTSE+$s(e)$ method, *i.e.* the ground state energy $e_0$ and the $T = 0$ magnetic susceptibility $\chi_0$, are discussed.

## CONTENTS

Introduction 2

I. High Temperature Series Expansions and their Padé approximants 3
A. The KHAF 4
B. Influence of impurities 5
C. Influence of a magnetic field 5
D. Influence of a Dzyaloshinskii–Moriya interaction 5
E. Influence of an Ising interaction 6
F. Influence of a second neighbor interaction $J_2$ 7
G. Influence of a third neighbor interaction $J_3$ 7
H. Influence of a third neighbor interaction $J_{3h}$ 8

II. HTSE+$s(e)$ and their Padé approximants 8
A. The use of $s(e,h)$ 8
B. The auxiliary function $G(e,h)$ 9
C. Specific heat $c_V$ 11
1. Raw $e$-HTSE and its Padé approximants 11
2. $c_V(T)$ from HTSE+$s(e)$ 11
D. Magnetic susceptibility $\chi(e)$ 11
1. Raw $e$-HTSE and its Padé approximants 11
2. $\chi(e)$ from HTSE+$s(e)$ 12
E. Coinciding Padé Approximants (CPAs) 13
F. Protocole to determine the best ground state energy 13

III. Attempt for a determination of $\chi_0$ 17
A. KHAF 17
B. Influence of impurities 18
C. Influence of Dzyaloshinskii–Moriya interaction 19
D. Influence of an Ising interaction 20
E. Influence a second neighbor interaction $J_2$ 21
F. Influence a third neighbor interaction $J_3$ 22
G. Influence a third neighbor interaction $J_{3h}$ 23

IV. Influence of perturbations on the KHAF 24
A. Influence of impurities 24
B. Influence of the magnetic field 26
C. Influence of Dzyaloshinskii–Moriya interaction 29
D. Influence of the Ising anisotropy 31
E. Influence of the second neighbor interaction $J_2$ 34
F. Influence of the third neighbor interaction $J_3$ 37
G. Influence of the third neighbor interaction $J_{3h}$ 40

## INTRODUCTION

First, we recall the Hamiltonian of a Heisenberg model with a constant magnetic field $B$ along the $z$-axis (Eq. (1) of the article):

$$\mathcal{H}_0 = J_1 \sum_{\langle i,j\rangle} \boldsymbol{S}_i \cdot \boldsymbol{S}_j, \qquad \mathcal{H} = \mathcal{H}_0 - hS^z, \tag{1}$$

where $\boldsymbol{S}_i$ are 1/2-spins, $S^z = \sum_i S_i^z$ is the total spin along the $z$-axis, and $h = g\mu_B B$. In the following we set $J_1 = 1$ (antiferromagnetic first neighbor interactions) and $g\mu_B = 1$. The partition function, $Z$, of a $N$-spin system is, with

$\beta = 1/T$:

$$Z = \text{Tr}\, \exp(-\beta\mathcal{H}) \tag{2}$$

$$= \sum_{S_z=-N/2}^{N/2} e^{-\beta h S_z} \text{Tr}_{\text{S}_\text{z}}\, \exp(-\beta\mathcal{H}_0), \tag{3}$$

where $\text{Tr}_{\text{S}_\text{z}}$ is the trace over the spin states of fixed $S_z$.

The free energy per spin, $f$, is defined as $-\beta f = \frac{1}{N}\ln Z$. The specific heat, $c_V(T)$, magnetization, $m$, and magnetic susceptibility, $\chi(T)$, per spin are defined as:

$$c_V(T,h) = \frac{1}{N}C_V(T,h) = -\beta^2 \left.\frac{\partial^2 \beta f(\beta,h)}{\partial\beta^2}\right|_h \tag{4}$$

$$m(t,h) = \left.\frac{\partial f(\beta,h)}{\partial h}\right|_\beta \tag{5}$$

$$\chi(T,h) \simeq \frac{m(T,h)}{h} \tag{6}$$

Note that we use here the magnetic susceptibility that is the more easily experimentally measured: $m(T,h)/h$ and not the derivative $\partial m(T,h)/\partial h$.

The HTSE (High Temperature Series Expansion) of the basic quantity $f$ in the thermodynamic limit reads

$$-\beta f(\beta,h) = \lim_{N\to\infty} \frac{1}{N}\ln Z(\beta,t)$$

$$= \ln 2 - \ln(1-t^2)/2 + \sum_{i=0}^{n} \beta^i \sum_{k=0}^{i} L_{ik} t^{2k}, \tag{7}$$

where $t = \tanh(\beta h/2)$, and the first two terms in Eq. (7) stand for the free spin contributions, while the last one comes from $\mathcal{H}_0$ and $L_{ik}$ are numbers. In Eq. (7), the sum over $k$ accounts exactly for the magnetic field. In the following, we expand $t$ in $\beta h$ and chose an order in $\beta$ above which terms are truncated.

From now, the spins are on a kagome lattice and we call KHAF the first neighbor antiferromagnetic Heisenberg model on this lattice, defined in Eq. (1).

In Sec. I, we give the HTSE results and its Padé approximants (PAs) for the KHAF and for this model submitted to various perturbations: impurities, magnetic field, Dzyaloshinskii–Moriya interaction, Ising interaction, second neighbor interaction and third neighbor interaction. $c_V(T)$ and $\chi(T)$ are shown in this first section. Here, only HTSE's are used and no information on the ground state is provided to bias the PA extrapolations.

In Sec. II we recall the steps followed in the HTSE+$s(e)$ method to extrapolate thermodynamic quantities over the full temperature range. We first replace the variable $\beta$ by the energy $e$ through a Legendre transform, leading to series in $e$ ($e$-HTSE). A direct use of the $e$-HTSE is possible for $\chi$ (Sec. II D 1), but the entropy method rests on an extrapolation of the entropy $s(e,h)$ using an auxiliary function (Sec. II B). $c_V$ and $\chi$ are then obtained from the derivatives of $s(e,h)$ with respect to $e$ for $c_V$ and with respect to the magnetic field $h$ for $\chi$. A model for the function $s$ is used which depends on the ground state energy $e_0$. At the end of this section, we propose a protocole to estimate $e_0$ when it is unknown.

In the presence of a magnetic field $h$, the variation of $e_0(h)$ with $h$ can be used to estimate the zero temperature and zero field magnetic susceptibility $\chi_0$. Two possibilities arise: either we chose $\chi_0$ as an hypothesis on the ground state and deduce $e_0(h)$ from it, or we use the protocole described previously to estimate $e_0(h)$ at different $h$ and extract $\chi_0$ from it. This last possibility is explored in Sec. III and the effect of the above perturbations on the $\chi_0$ estimation is determined.

The last section (IV) is devoted to the effects of the above perturbations on $c_V(T)$ and $\chi(T)$ through HTSE+$s(e)$.

## I. HIGH TEMPERATURE SERIES EXPANSIONS AND THEIR PADÉ APPROXIMANTS

From the HTSE of $\frac{1}{N}\ln Z(\beta,h)$ (Eq. (7)) at order $n$ and Eqs. (4)-(5), we deduce the HTSE of $c_V(T)$ at the same order and of $\chi(T)$ at order $n-1$. In this section, we directly exploit the raw series coefficients of the $c_V(T)$ and $\chi(T)$ functions by representing and studying the convergence of: $i$) the truncated series and $ii$) their Padé approximants (PAs). We do not use any (known or supposed) physical information on for example the nature of the ground state, which will be the subject of the next sections. Sub-section I A shows the results obtained for the KHAF and the next ones (I B to I H) analyze the effects of perturbations on it.

## A. The KHAF

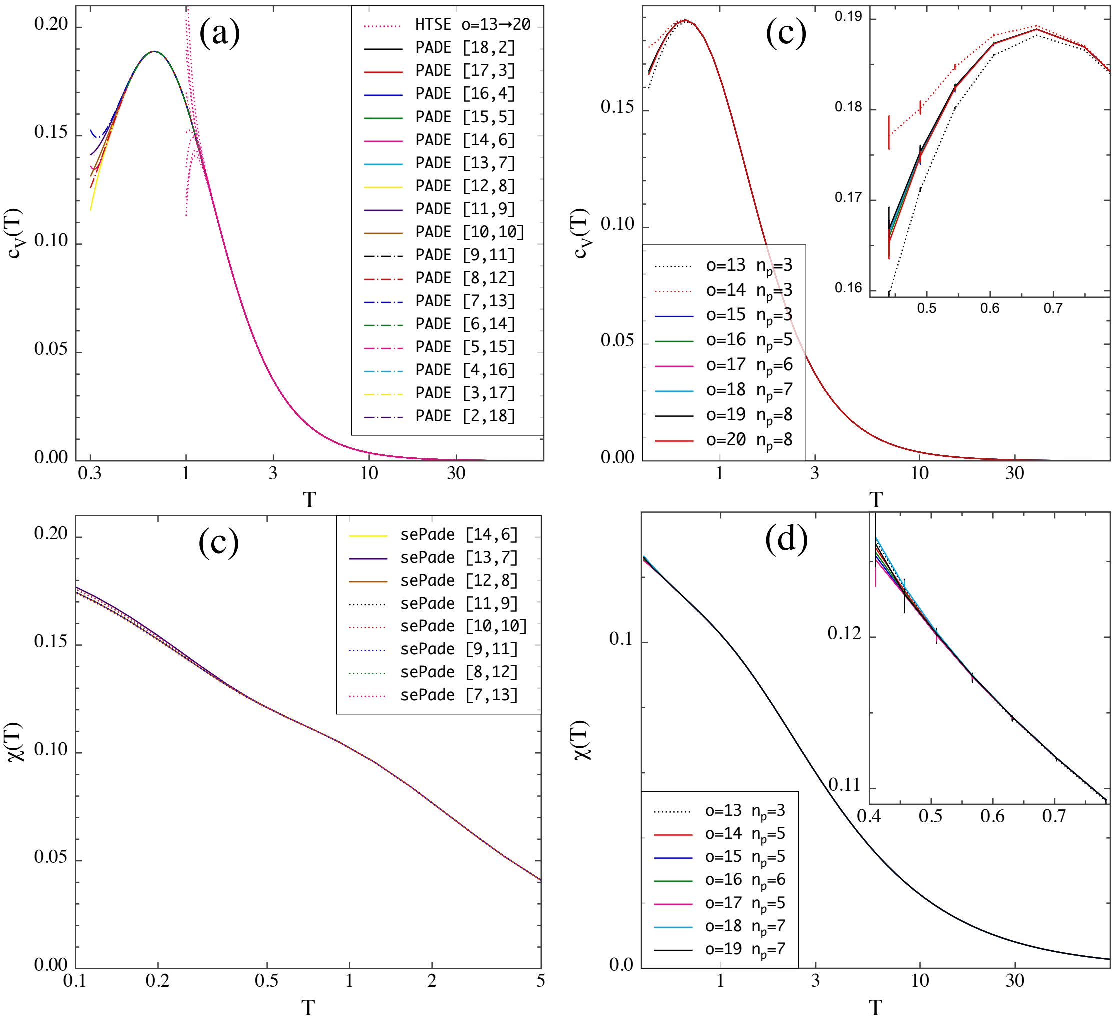


FIG. 1. (a) HTSE and PAs of $c_V(T)$ at $h = 0$ for the KHAF model. Dotted red lines stand for the raw series at orders from 13 to 20. Full and dash-dot lines are the PAs of the HTSE at order 20. (b) CPAs of the HTSE of $c_V(T)$ at order $o$ from 13 to 20, where $n_p$ indicates the number of coinciding PAs within a distance of 0.004 (see Sec. II E). Error bars in the insets indicate the dispersion of the CPAs. (c) and (d) same as (a) and (b) for $\chi(T)$ except that the maximum order is now 19.

The HTSE of $c_V(T, h = 0)$ (red dotted lines) converge for $T > 1.3$. They are shown on Fig. 1-(a) for orders from 13 to 20. For each order, we can construct a collection of PAs, labelled by $[p, q]$ with $p$ the numerator and $q$ the denominator degree. Among them, on a fixed interval of temperature, some are unphysical and are eliminated (for example, with negative values of $c_V$). Several of the remaining ones can be coinciding Padé approximants (CPAs) (see Sec. II E for the precise definition). Their number for a given distance is called $n_p$. Among the PAs of the HTSE at order 20 (Fig. 1-(a)), we see CPAs for $T > 0.45$: here, the CPAs have denominator degrees from 7 to 14. The convergence of the $c_V$-CPAs is improved going from order 13 to 20, winning a factor 2 in the range of temperatures (Fig. 1-(b)).

The same study is now done for $\chi(T)$ at $h = 0$, for HTSE orders from 13 to 19. The HTSE of $\chi(T)$ converge for $T > 1.05$ (Fig. 1-(c)) For $T > 0.45$, the CPAs of the HTSE at order 19 have also denominator degrees from 7 to 14 (Fig. 1-(c)). In the inset of Fig. 1-(d), we see that the $\chi$-CPAs obtained from different orders start to diverge for $T < 0.5$.

In the next sub-section, only the CPAs for the largest order series will be presented, with $n_p$ as an indication of the results fiability.

### B. Influence of impurities

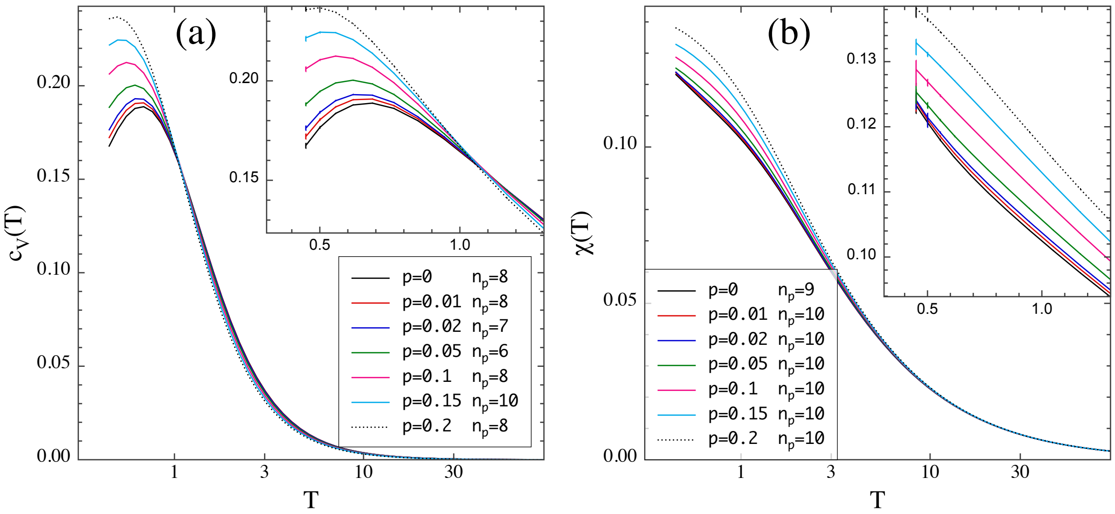


FIG. 2. KHAF model with an impurity rate $p$ at $h = 0$. (a) CPAs of $c_V(T)$ from HTSE at order 20. (b) CPAs of $\chi(T)$ from HTSE at order 19. Insets are zooms where the error bars show the dispersion of the CPAs.

Impurities have been accounted in the HT-series in a statistical way. Each graph made of $m$ sites gets a weight $q^m$, where $q = 1 - p$ and $p$ is the probability that a spin is missing. Thus we take into account the missing spins, but not the additional spins that can be elsewhere. The actual HT-series is now also a polynomial of $q$ starting at order 2 for the exchange part (the smallest diagram with exchange contains two spins). The total number of spins is thus proportional to $q$. Then, Eq. (7) for the partition function per spin (and not per site) becomes:

$$-\beta f(\beta, h) = \ln 2 - \frac{\ln(1-t^2)}{2} + \frac{1}{q}\sum_{j=2}^{j_{\max}} q^j \sum_{i=0}^{n} \beta^i \sum_{k=0}^{i} L_{j,i,k} t^{2k}, \tag{8}$$

where $L_{j,i,k}$ are numbers and $j_{\max}$ is the number of sites of the largest graphs. At order $n$, the largest graphs have a tree topology (the graphs found at the largest order in $k$) and their number of sites is $n+1$, thus $j_{\max} = n+1$.

We now look at the effect of impurities on the CPAs of $c_V(T)$ and $\chi(T)$ for the KHAF at $h = 0$ (Fig. 2). The effect starts at $T < 1$ for $c_V$ and $T < 3$ for $\chi$. Impurities increase the value of the maximum of $c_V(T)$ and slightly enhance $\chi(T)$ at the lowest temperatures shown here.

### C. Influence of a magnetic field

Above $T = 0.45$ a magnetic field $h \leq 0.2$ has negligible effects on $c_V(T,h)$ and $\chi(T,h)$ for the KHAF model. Effects start at a field of 0.5 at these temperatures. Thus a figure of the CPAs is meaningless in this subsection and the small changes due to $h$ in the series coefficients will only be visible at low temperatures and thanks to the HTSE+$s(e)$ method of the next sections.

### D. Influence of a Dzyaloshinskii–Moriya interaction

A Dzyaloshinskii–Moriya interaction (DMI) is added to the HKAF model of Eq. (1):

$$\mathcal{H}_{\rm DM} = \sum_{\langle i,j\rangle} D_z \left(\mathbf{S}_i \wedge \mathbf{S}_j\right)_z \tag{9}$$

The HTSE has been computed up to order 16 in $\beta$ in Eq. (7) after the Taylor expansion of $t$ in $\beta h$. A DMI enhances the peak of $c_V(T)$ for $h = 0$ (see Fig. 3-(a)). On the contrary, negligible effects are seen on $\chi(T)$ above $T = 0.45$ (see Fig. 3-(b)).

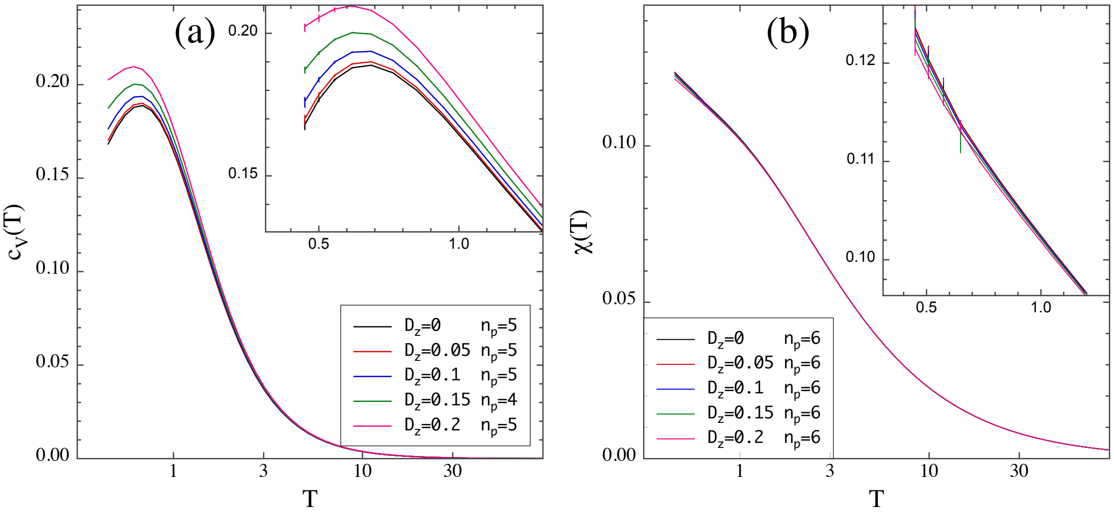


FIG. 3. KHAF model with a Dzyaloshinskii–Moriya interaction $D_z$ at $h = 0$. (a) CPAs of $c_V(T)$ from HTSE at order 16. (b) CPAs of $\chi(T)$ from HTSE at order 15. Insets are zooms where the error bars show the dispersion of the CPAs.

### E. Influence of an Ising interaction

An Ising anisotropy term is added to the HKAF model of Eq. (1):

$$\mathcal{H}_{\text{Ising}} = \sum_{\langle i,j \rangle} \delta_z S_{iz} S_{jz}. \tag{10}$$

The HTSE has been computed up to order 18 in $\beta$ in Eq. (7) after the Taylor expansion of $t$ in $\beta h$. $\delta_z$ has a small effect on $c_V(T)$ (Fig. 4-a). For $h = 0$, It causes a small shift of the position of the maximum of $c_V(T)$ to smaller temperature if $\delta_z < 0$, and to higher temperature if $\delta_z > 0$. Below $T = 3$, $\chi(T)$ is increased when $\delta_z$ decreases (Fig. 4-b).

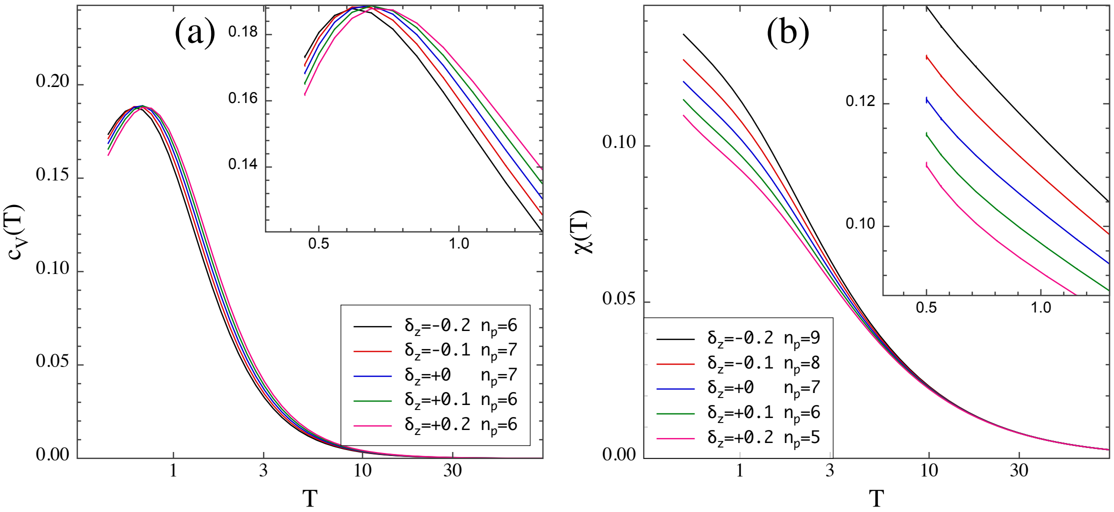


FIG. 4. KHAF wit an Ising interaction $\delta_z$ at $h = 0$. (a) CPAs of $c_V(T)$ from HTSE at order 18. (b) CPAs of $\chi(T)$ from HTSE at order 17. Insets are zooms where the error bars show the dispersion of the CPAs.

### F. Influence of a second neighbor interaction $J_2$

A second neighbor interaction, $J_2$ is added. The HTSE has been computed up to order 15 in $\beta$ in Eq. (7) after the Taylor expansion of $t$ in $\beta h$. At $h = 0$, a small $J_2$ has an effect for $T < 3$ both for $c_V(T)$ and $\chi(T)$ (Fig. 5).

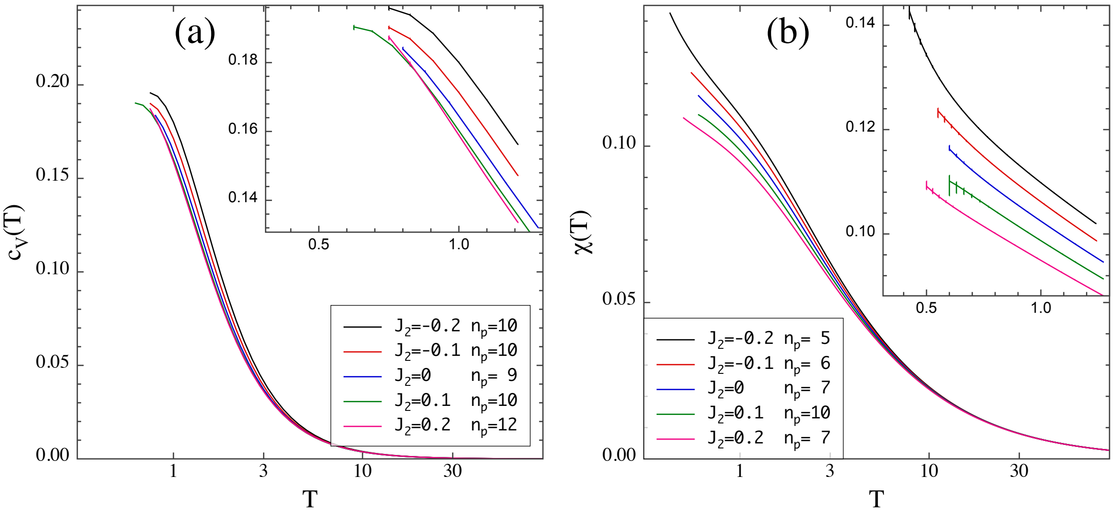


FIG. 5. KHAF with a second neighbor interaction, $J_2$ at $h = 0$. (a) CPAs of $c_V(T)$ from HTSE at order 15 (b) CPAs of $\chi(T)$ from HTSE at order 14. Insets are zooms where the error bars show the dispersion of the CPAs.

### G. Influence of a third neighbor interaction $J_3$

A third neighbor interaction, $J_3$, is added. The HTSE has been computed up to order 15 in $\beta$ in Eq. (7) after the Taylor expansion of $t$ in $\beta h$. At $h = 0$, a small $J_3$ has an effect for $T < 3$ both for $c_V(T)$ and $\chi(T)$ (Fig. 6-(a)). A small $J_3$ has a *linear* effect on $\chi(T, h = 0)$ for $T < 3$ (see Fig. 6-(b)).

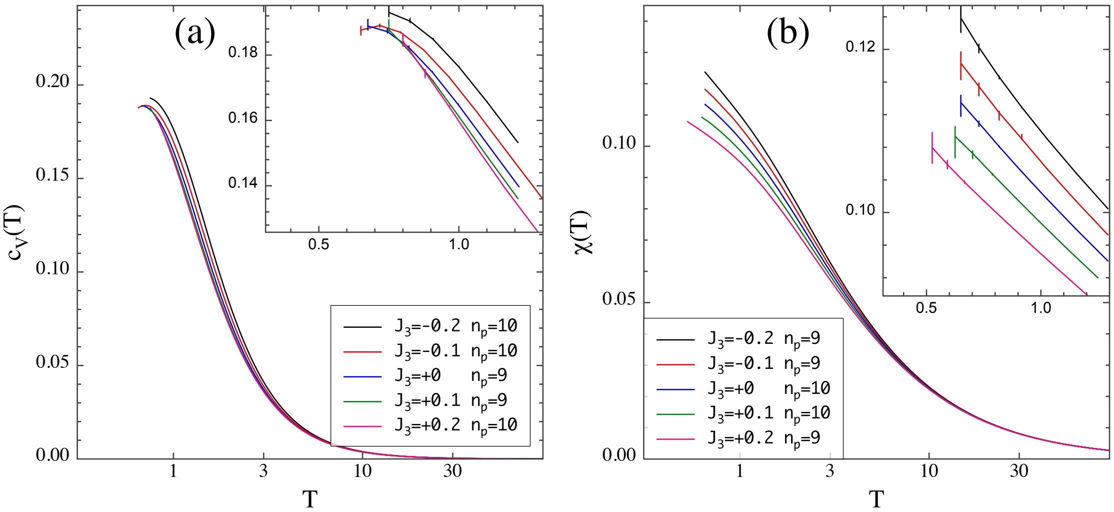


FIG. 6. KHAF with a third neighbor interaction $J_3$ at $h = 0$. (a) CPAs of $c_V(T)$ from HTSE at order 15 (b) CPAs of $\chi(T)$ from HTSE at order 14. Insets are zooms where the error bars show the dispersion of the CPAs.

### H. Influence of a third neighbor interaction $J_{3h}$

A third neighbor interaction across the hexagon, $J_{3h}$, is added. The HTSE has been computed up to order 15 in $\beta$ in Eq. (7) after the Taylor expansion of $t$ in $\beta h$. A small negative $J_{3h}$ has almost no effect on $c_V(T, h = 0)$, and increases slightly its maximum for positive $J_{3h}$ (see Fig. 7-(a)). A small $J_{3h}$ has a *linear* effect on $\chi(T, h = 0)$ for $T < 3$ (see Fig. 7-(b)). While $J_3$ and $J_{3h}$ have opposite effects on $c_V(T)$, they have similar effects on $\chi(T)$.

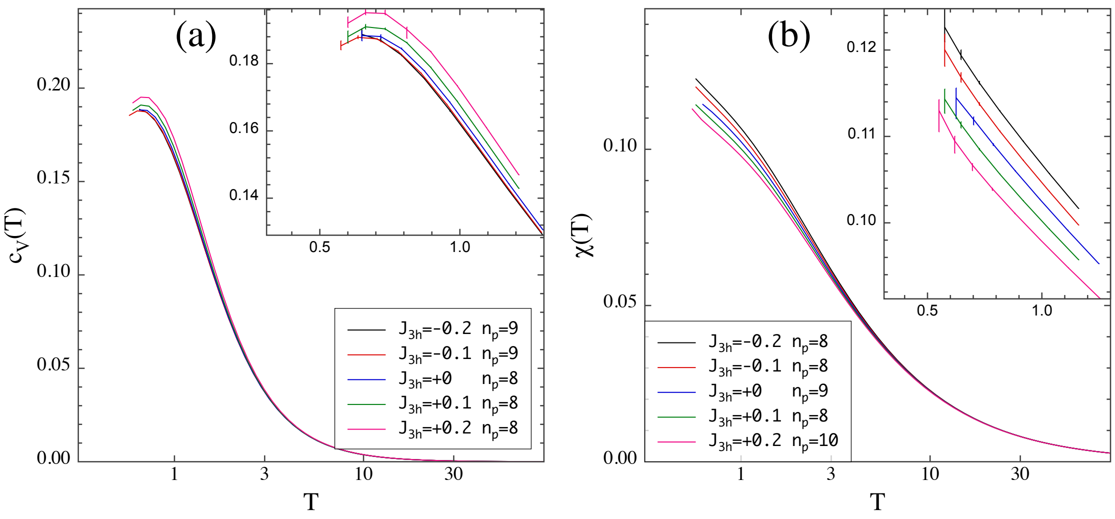


FIG. 7. KHAF with a third neighbor interaction across the hexagon $J_{3h}$ at $h = 0$. (a) CPAs of $c_V(T)$ from HTSE at order 15 (b) CPAs of $\chi(T)$ from HTSE at order 14. Insets are zooms where the error bars show the dispersion of the CPAs.

## II. HTSE+$s(e)$ AND THEIR PADÉ APPROXIMANTS

The studies of the raw HTSE's and of their direct PAs show that the convergence of $c_V(T)$ and $\chi(T)$ is limited to temperatures of the order of $J_1$ for the raw series, and of $J_1/2$ for the PAs. We now describe the HTSE+$s(e)$ method that extends the range of convergence down to zero temperature at the price of imposing some conditions on the extrapolation, assuming that no transition occurs at any temperature, *i.e.* that all functions are analytic.

### A. The use of $s(e, h)$

We first perform a Legendre transformation of $\frac{1}{N} \ln Z$. The temperature $T$ is replaced by the energy per site $e$:

$$e = -\frac{1}{N} \left. \frac{\partial \ln Z(\beta, h)}{\partial \beta} \right|_h . \tag{11}$$

The new relevant thermodynamic function is the entropy per site $s$:

$$s(e, h) = \frac{1}{N} \ln Z(\beta, h) + \beta e. \tag{12}$$

Eliminating $\beta$ in Eq. (12) using the HTSE of $\frac{1}{N} \ln Z$ gives the $e$-HTSE for $s(e, h)$. In practice, $h$ is always replaced by some number $h_0$ in Eqs.(11)-(12) and (7) before $s(e, h_0)$ is evaluated. From this function the specific heat and magnetic susceptibility are given by:

$$c_V(e, h_0) = -\frac{s'(e, h_0)^2}{s''(e, h_0)} \tag{13}$$

$$\chi(e, h_0) \simeq \frac{m(e, h_0)}{h_0} = \frac{1}{\beta h_0} \left. \frac{\partial s(e, h)}{\partial h} \right|_{e, h=h_0} , \tag{14}$$

where $s'$ and $s''$ mean the first and second derivatives of $s(e,h)$ with respect to $e$. We evaluate the $h$-derivatives from finite differences. At $h \neq 0$, we have

$$\left.\frac{\partial s(e,h)}{\partial h}\right|_e = \frac{s(e,h+dh) - s(e,h-dh)}{2dh} + O(dh^2), \tag{15}$$

while at $h = 0$:

$$\lim_{h\to 0} \frac{1}{h}\left.\frac{\partial s(e,h)}{\partial h}\right|_e = 2\frac{s(e,dh) - s(e,0)}{dh^2} + O(dh^2) \tag{16}$$

and

$$\chi(e,h=0) \simeq 2\frac{s(e,dh) - s(e,0)}{\beta dh^2}. \tag{17}$$

$dh$ is typically of the order of $10^{-4}$.

By definition $\beta = s'(e,h))$, thus $s(e,h)$ must be a positive increasing function. Because $c_V$ is also positive, then $s''(e,h)$ must be negative. Thus $s(e,h)$ is an increasing and concave function starting at $s = 0$ for $e = e_0(h)$, the ground state energy, with an infinite slope and ending at $s = \ln 2$ when $e = 0$ with a slope 0.

The next step is to build a procedure to extrapolate $s(e,h)$ using the HTSE and the type of singularity of $s$ at $e = e_0(h)$, given by the low-$T$ behavior of $c_V$. The next sub section shows a way to remove this singularity using an auxiliary function, assuming that no other singularity exists between $e = 0$ and $e_0(h)$.

We assume either a non-gapped system where

$$c_V(T) \propto T^\alpha \tag{18}$$

or a gapped system where

$$c_V(T) \propto T^2 e^{-\delta/T}. \tag{19}$$

In the following we systematically test the cases $\alpha = 1$ and 2, and the gapped case, which will be denoted $\alpha = 0$.

### B. The auxiliary function $G(e,h)$

- We first consider the ungapped case. A power law behavior of $c_V$ in $T^\alpha$ at low $T$ implies a singular behavior of $s(e,h)$ at the ground state energie $e_0(h)$:

$$s(e,h) \propto (e - e_0(h))^{1/\mu}, \qquad \mu = 1 + \frac{1}{\alpha}. \tag{20}$$

  This singularity at $e_0$ prevents us to directly use the $e$-HTSE of $s(e,h)$. Instead, we use the $e$-HTSE of an auxiliary function $G(e,h)$ depending on $s(e,h)$ and defined by:

$$G(e,h) = \frac{s(e,h)^\mu}{e - e_0(h)}, \tag{21}$$

  If no transition occurs in the whole range of temperatures, then $G(e,h)$ should be a constant sign regular function of $e$. The $e$-HTSE of $G(e,h)$ is deduced from the $e$-HTSE of $s(e,h)$ (note that $G(e,h)$ depends on the choice of $e_0(h)$ through Eq. (21)). Then, the PAs $G_{\rm PA}(e,h)$ are constructed, from the $e$-HTSE of $G(e,h)$, and the function $s_{\rm PA}(e,h)$ is approximated by:

$$s_{\rm PA}(e,h) = \left(G_{\rm PA}(e,h)(e - e_0(h))\right)^{1/\mu}. \tag{22}$$

- For a gapped ground state, the main singularity of $s(e,h)$ around $e_0$, here independent of $h$ at least for not too large $h$, reads

$$s(e,h) \propto (e - e_0)\ln(e - e_0). \tag{23}$$

To account for it, on way is to define an auxiliary function $G(e,h)$:

$$G(e,h) = \left(\frac{s(e,h)}{e-e_0}\right)'(e-e_0), \tag{24}$$

where the prime means the derivative with respect to $e$. Similarly to the ungapped case, the PAs $G_{\rm PA}(e,h)$ are constructed from the $e$-HTSE of Eq. 24, and the function $s(e,h)$ is approximated by:

$$s_{\rm PA}(e,h) = (e-e_0)\left(-\frac{\ln 2}{e_0} - \int_e^0 d\varepsilon\, \frac{G_{\rm PA}(\varepsilon,h)}{\varepsilon - e_0}\right) \tag{25}$$

By construction, $s_{\rm PA}(e,h)$ has the exact $e$-HTSE and the correct low energy behavior. Fig. 8 shows the convergence of the $e$-HTSE of $G(e,h)$ and of $G_{\rm PA}(e,h)$, for $\alpha = 0$, 1 and 2. While the raw series converge slowly at low energy, their PAs are well converged down to $e_0$.

The function $G(e,h)$ depends on the ground state energy $e_0(h)$ (Eq. (21) or (24) and Fig. 8-(b)). The sensibility of $G(e,h)$ to $e_0(h)$ is important only at low energies. We measure the number of CPAs by keeping the PAs whose maximum distance between them is some $\Delta$ and call their number $n_p$. For $\alpha = 0$, the maximum of $n_p$ for $\Delta = 0.1$ is for $e_0 \simeq -0.437$. For $\alpha = 1$, it is for $e_0 \simeq -0.438$ and for $\alpha = 2$ for $e_0 \simeq -0.441$.

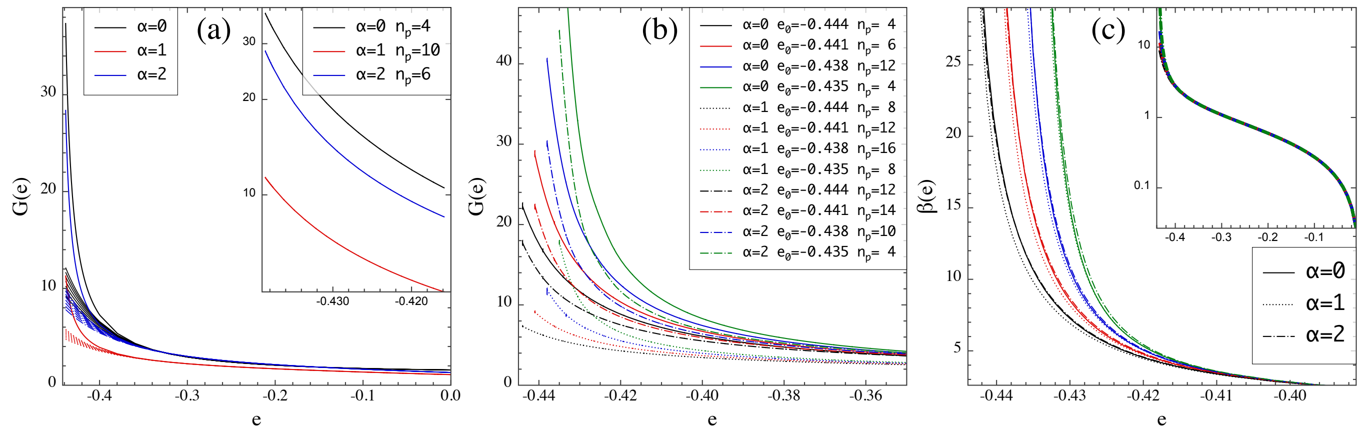


FIG. 8. Auxiliary function $G(e)$ ($-G(e)$ for $\alpha = 0$) from for the KHAF at $h = 0$. (a) $e$-HTSE from order 13 to 20 (dotted lines) and CPAs (full lines) for $\alpha = 0$ (black), 1 (red) and 2 (blue) with the hypothesis $e_0 = -0.4386$. Inset: zoom of the CPAs around $e_0$. $n_p$ is the number of CPAs within a distance $\Delta = 0.1$. (b) CPAs of $G(e)$ from various values of $e_0$ around the ground state energies for $\alpha = 0$ (full lines), 1 (dotted lines) and 2 (dashed-dotted lines). (c) $\beta(e)$ as defined by Eq. (26), from results of (b) (same colors). Inset: all curves coincide as soon as $\beta < 3$ ($e \gtrsim -0.4$).

The entropy is defined from the CPAs of $G(e)$ by Eqs. (22) and (25), and the inverse temperature is given by:

$$\beta(e) = \frac{1}{T(e)} = s'_{\rm PA}(e) \tag{26}$$

For $e > -0.4$, $\beta(e)$ is rather independent of $\alpha$ and of $e_0$ (see Fig. 8-(c)). It corresponds to $\beta \gtrsim 3$, that is $T \gtrsim 0.33$. For $e < -0.4$, $\beta(e)$ begins to be sensitive to $e_0$, but much less to $\alpha$ (see Fig. 8-(c)).

The value $G(e_0)$ is directly related to a temperature $T_0$, characteristic of the low-$T$ behavior of $c_V(T)$, as for example the inverse of the gap for $\alpha = 0$:

$$C_V(T) \propto T^2 e^{-T_0/T} \Rightarrow T_0 = -\frac{1}{G(e_0)} \qquad \text{gapped systems} \tag{27}$$

$$C_V(T) \simeq \frac{T}{T_0} \Rightarrow T_0 = \frac{2}{G(e_0)} \qquad \alpha = 1 \tag{28}$$

$$C_V(T) \simeq \left(\frac{T}{T_0}\right)^2 \Rightarrow T_0 = \frac{3}{2\sqrt{2}\,G(e_0)} \qquad \alpha = 2 \tag{29}$$

$$C_V(T) \simeq \left(\frac{T}{T_0}\right)^\alpha \Rightarrow T_0 = \frac{\alpha+1}{\alpha^{1+1/\alpha}\,G(e_0)} \qquad \alpha > 0. \tag{30}$$

$T_0$ will be given for all the extrapolations of Sec. IV for the three cases $\alpha = 0$, 1 or 2.

## C. Specific heat $c_V$

### 1. Raw e-HTSE and its Padé approximants

From Eq. (4) and (7), we can deduce the HTSE for $c_V(T)$ and then the $e$-HTSE for $c_V(e)$ from the HTSE of $e(\beta)$. Near $e_0$, the behavior of $c_V(e)$ is:

$$\begin{array}{ll} c_V(e) \sim -G(e_0)(e-e_0)(\ln(e-e_0))^2 & \text{for gapped systems} \\ c_V(e) \sim \alpha G(e_0)^{1/\mu}(e-e0)^{1/\mu} & \text{for } \alpha > 0, \end{array}$$

with a singular behavior that cannot been obtained through $e-$HTSE. However, the $e-$HTSE and their PAs are represented on Fig. 9.

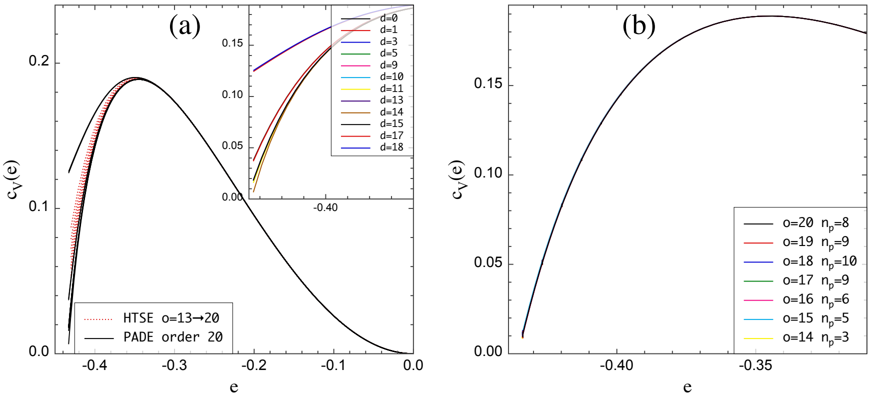


FIG. 9. $c_V(e)$ from $e$-HTSE. (a) Red dotted lines: $e$-HTSE at orders $o = 13$ up to 20. Full lines: PAs from $e$-HTSE at order 20. Inset: zoom at low energy. (b) CPAs obtained for orders 14 to 20 of the $e$-HTSE, where the error bars indicate the dispersions of the PAs. The energies have been slightly shifted to see the error bars.

### 2. $c_V(T)$ from HTSE+$s(e)$

The HTSE+$s(e)$ specific heat is given from $s_{\rm PA}(e,h)$ as:

$$c_V(e,h) = -\frac{s'_{\rm PA}(e,h)^2}{s''_{\rm PA}(e,h)}. \qquad (31)$$

From $\beta(e,h)$ (Eq. (26)), we can change the variable $e$ to $T$ and get the function $c_V(T)$. From Fig. 8-(c), we do not expect differences for $T > 0.35$ in $c_V(T)$ by varying $e_0$ or $\alpha$. Fig. 10 shows the variations of $c_V(T)$ and $c_V(e)$ at $h = 0$ using HTSE, the PAs of HTSE at order 20 and HTSE+$s(e)$ (Eq. (31)) for $e_0 = -0.4386$.

## D. Magnetic susceptibility $\chi(e)$

### 1. Raw e-HTSE and its Padé approximants

From Eq. (5) and (7), we deduce the HTSE for $\chi(T)$. From the HTSE of $e(\beta)$ and $\chi(\beta)$, we deduce the $e$-HTSE for $\chi(e)$. In contrast with $c_V(e)$, $\chi(e)$ does not a present singular behavior at low energy, thus the function $\chi(e)$ should be smooth if no transition occurs. Fig. 11-(a) shows the convergence of the $e$-HTSE with the order (from 13 to 19) down to $e \simeq -0.3$, and PAs obtained at the highest order 19. The PAs from $e$-HTSE at orders $n \geq 13$ all have almost the same variations, namely a pronounced increase at low energies (Fig. 11-(b)). As the PAs seem to converge down to the expected ground state energy, this indicates a possible large value of $\chi$ at low energy (low $T$).

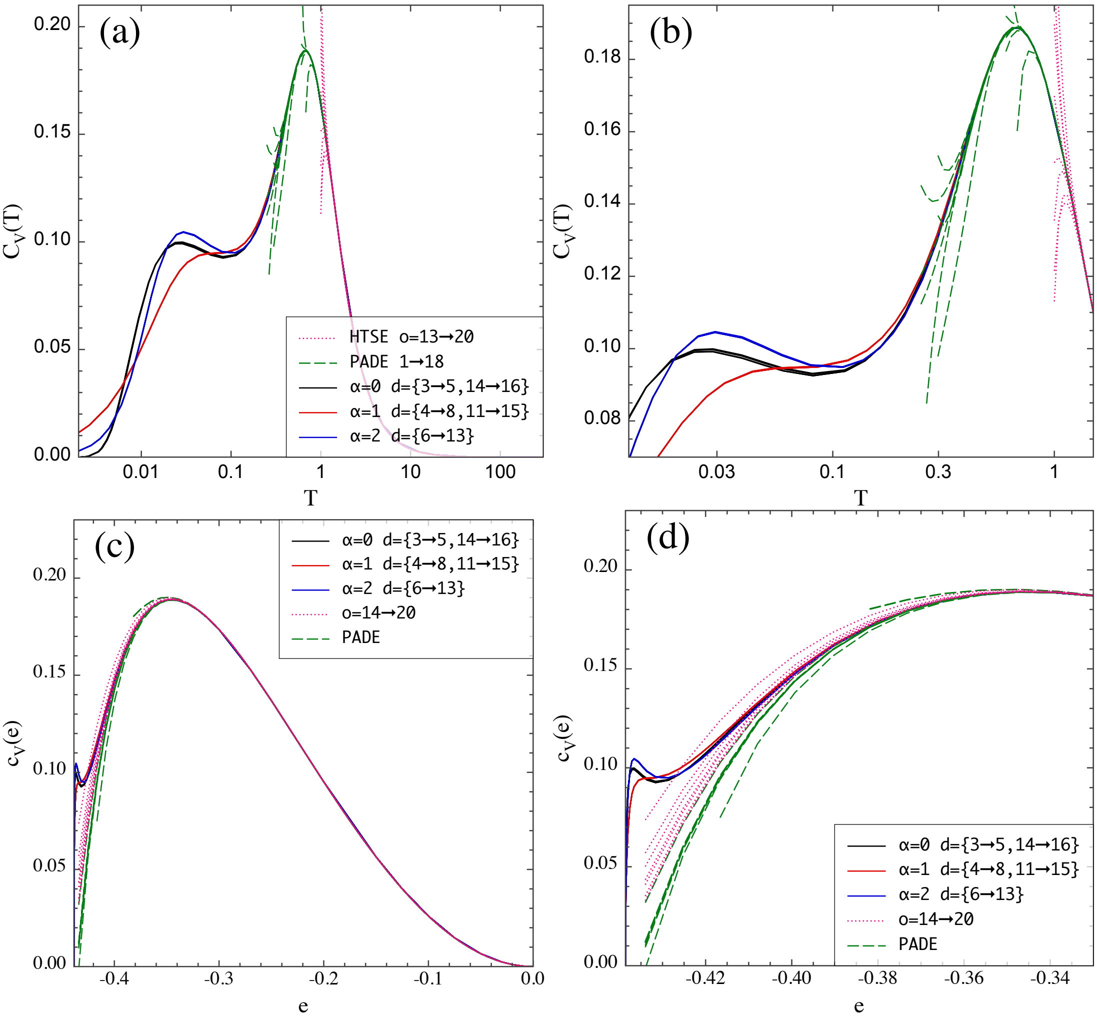


FIG. 10. (a): $c_V(T)$ of the KHAF for $h=0$; HTSE (order 14 to 20): dotted magenta lines; PADE means PAs [20-d,d] of HTSE at order 20 for $d$=1 through 18 excepted d=2, 6, 7, 8, 12 which have a pole: dashed green lines HTSE+$s(e)$ results (from Eq. (31)) for $e_0=-0.4386$ (only CPAs are represented): black (resp. red, blue) full lines for $\alpha=0$ (gapped) (resp. $\alpha=1$, 2). (b): zoom of (a). (c): $c_V(e)$ same data as (a) but with respect to $e$. (d): zoom of (c);

### 2. $\chi(e)$ from HTSE+$s(e)$

$\chi(e)$ is obtained using Eqs. (14), with $s(e,h)$ obtained from Eq. (22). The ground state energy $e_0(h)$ is required in these steps. For gapped systems, $\chi(T=0)=0$ and $e_0$ does not depend on $h$, while for non gapped systems, at small magnetic field, the ground state energy depends on $h$ as

$$e_0(h) = e_0 - \chi_0\frac{h^2}{2} + .. \tag{32}$$

where $\chi_0=\chi(T=0)$ is unfortunately unknown. Fig. 12 shows how the $\chi(T)$ obtained from HTSE+$s(e)$depends on $\chi_0$ for $\alpha=1$ and 2, at the highest order 20 for $e_0=-0.4386$. By construction both high (same HTSE) and low temperatures (same $\chi_0$) do not depend on $\alpha$. The main differences appear around $T=0.1$ for $\chi_0$ between 0.05 and 0.15. On Fig. 12-(b), we see that the convergence of the PAs from the HTSE converge for $T>0.5$. All variations of $\chi(T)$ using the various input $\chi_0$ and $\alpha$ are compatible with these PAs from HTSE.

For completeness, Fig. 12-(c) shows the comparison of $\chi(e)$ obtained from $s(e,h)$ with the direct $e$-HTSE of $\chi(e)$ and the PAs obtained from this $e$-HTSE at order 19.

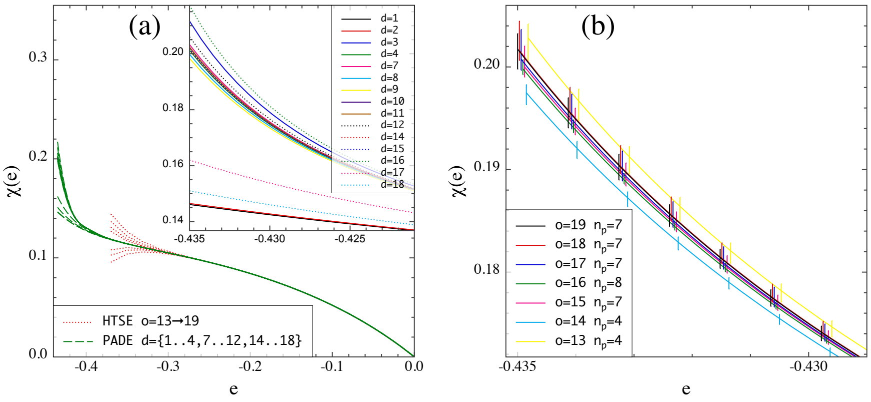


FIG. 11. $\chi(e)$ from $e$-HTSE. (a) Red dashed lines: $e$-HTSE at orders $o = 13$ up to 19. Full lines: PAs from $e$-HTSE at order 19. Inset: zoom at low energy, the PA $d = 0$ is outside of this inset. CPAs within a distance $\Delta = 0.004$ are for $d = 4$, 7, 8, 10, 11, 14, 15. (b) CPAs obtained for orders 13 to 19 of the $e$-HTSE, where the error bars indicate the dispersions of the PAs. The energies have been slightly shifted to see the error bars.

### E. Coinciding Padé Approximants (CPAs)

We define a procedure to find the coinciding PAs (CPAs) as follow. First we evaluate the function (say $c_V(T)$) obtained from each physical PA of the auxiliary function $G(e)$ on a grid of temperatures, using an interpolation scheme (recall that the PAs are functions of $e$). We can keep the PAs from several HTSE orders. Then, we apply the loop:

- evaluate the average of all these functions on the $T$-grid,
- eliminate the function with the largest distance to the mean function,
- stop the loop when largest distance to the mean function is smaller than some threshold $\Delta$.

Fig. 13-(a) shows all the 68 physical PAs obtained from the orders 17 thru 20 with $e_0 = -0.4386$. Fig. 13-(b) shows the resulting 40 CPAs when $\Delta = 0.001$.

### F. Protocole to determine the best ground state energy

The ground state energy, $e_0$, is often unknown. Here we propose a protocole to estimate $e_0$, again based on the idea that larger is number of CPAs, best is its estimation. The CPAs are evaluated from the HTSE at different orders to account for the convergence of the PAs with the HTSE order. This is possible if the order $n$ of the HTSE is large enough to avoid a shift of the PAs with respect to $n$. Here, for $c_V(T)$, we already see a good convergence using the HTSE at order 17 through 20. Thus, we look at all the PAs at these orders (see Fig. 13). We keep the PAs obtained from the highest four HTSE-orders.

The protocole consists in the following steps:

- For a given $e_0$, evaluate the physical PAs from the highest HTSE-orders. The discarded non physical PA are those with a zero either in the numerator or denominator of the PA within the interval $[e_0, 0]$.
- Look for the CPAs at a given distance $\Delta$, as described in the previous section, and count their number $n_{\rm CPA}(e_0)$.
- Vary $e_0$ and define the best energy as that corresponding to the maximum of $n_{\rm CPA}(e_0)$. The precision of this determination is related to the width of $n_{\rm CPA}(e_0)$, say the interval defined by $n_{\rm CPA}(e_0) > \max(n_{\rm CPA}(e_0)) - 5$.

This protocole is tested on $c_V(T)$. Fig. 14-(a)(b)(c) shows how $n_{\rm CPA}$ varies with $e_0$ for $\Delta$ from $10^{-4}$ to 0.02, for $\alpha = 0$, 1 and 2. The best $e_0$ (maximum of $n_{\rm CPA}(e_0)$) is almost independent from $\Delta$, as evidenced in Fig. 14-(d). Using $\Delta = 0.001$ is a good compromise between selecting close curves and having a large number of CPAs. This gives a hint on the precision of such an evaluation of $e_0$. For $\alpha = 0$ (resp. 1 and 2), we find $e_0 \simeq -0.4372\,(15)$ (resp. $e_0 \simeq -0.4386\,(15)$ and $e_0 \simeq -0.4414\,(25)$). Note that this estimation of $e_0$ is compatible with the DMRG result -0.4386(5) for $\alpha = 1$, while we find a slightly higher energy for $\alpha = 0$ and a significant lower one for $\alpha = 2$.

The same protocole is also applied on $\chi(T)$. Here for each $\alpha = 0$, 1 and 2 and each value of $\chi_0 = 0$, 0.05, 0.1, 0.15 and 0.2 (only $\chi_0 = 0$ for $\alpha = 0$), we evaluate $n_{\rm CPA}(e_0)$ for different $\Delta$ (Fig. 15). The *best* $e_0$ versus $\Delta$ depends very

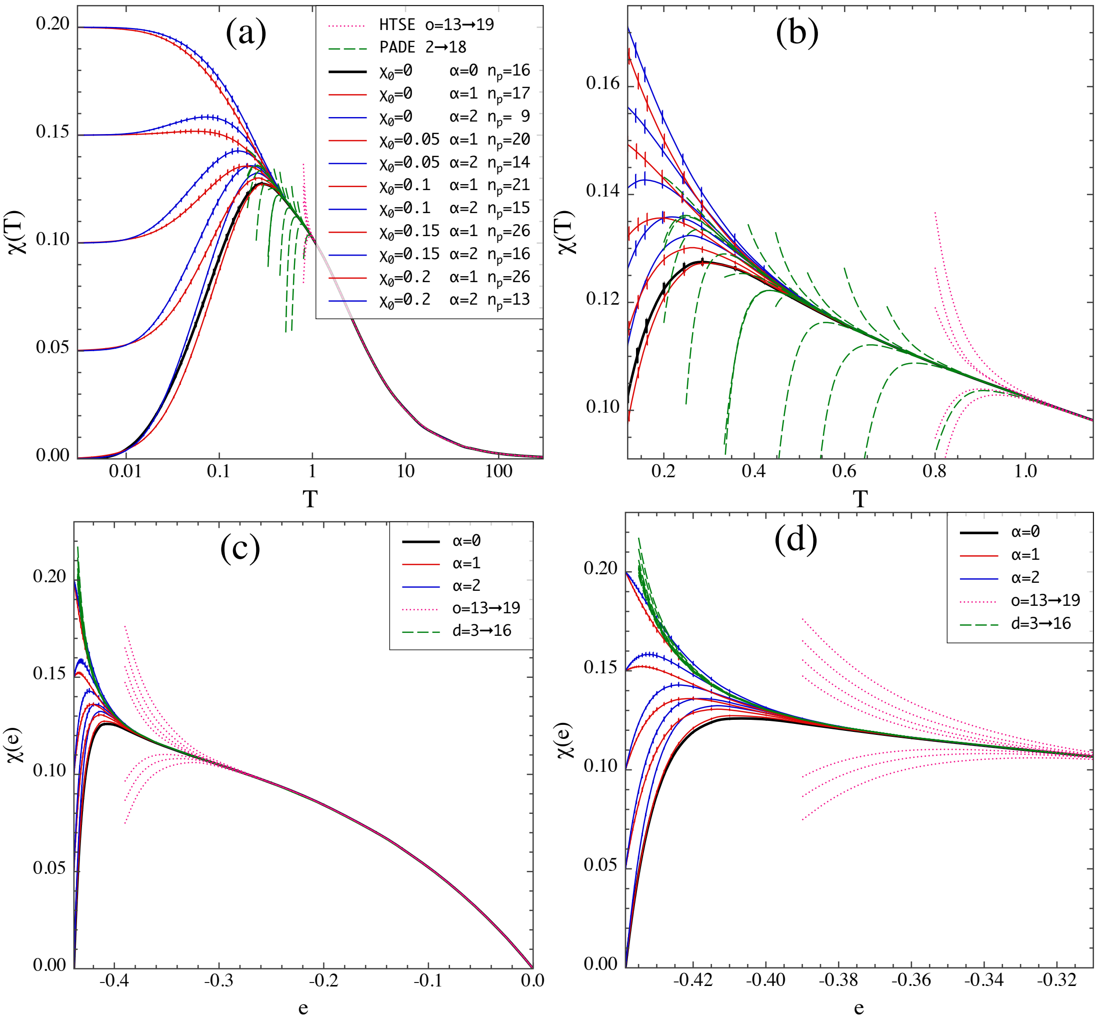


FIG. 12. (a) and (b) $\chi(T)$ for $e_0 = -0.4386$ and $\chi_{=}$0, 0.05, 0.1, 0.15 and 0.2. HTSE of $\chi(T)$ (dash-dot magenta lines) and its PAs (green dots). $\chi$ from HTSE+$s(e)$ (full lines) for $\alpha = 0$ (black), 1 (red) and 2 (blue). (b) is a zoom of (a) for $0.12 < T < 1.2$. (c) and (d) Same data as (a) and (b) versus e; dotted magenta lines: $e$-HTSE; green lines: PAs of $e$-HTSE at the highest order 19.

little on $\chi_0$ (see the last three figures of Fig. 15). In all cases the ground state energy obtained for $c_V$ is compatible with that of $\chi$ within their respective uncertainties.

Within uncertainties, one can assume the $e_0$ found from the CPAs of $\chi(T)$ to be independent of $\chi_0$ (Fig. 16). Thus for simplicity, in the following, the best $e_0$ will be evaluated for $c_V$ only and used for $\chi$ independently of $\chi_0$.

Note that when the HTSE is known at much lower orders, as for example for the $J_1$-$J_2$ or $J_1$-$J_{3h}$ models, the best ground state is evaluated with this low order series even when $J_2 = 0$ or $J_{3h} = 0$.

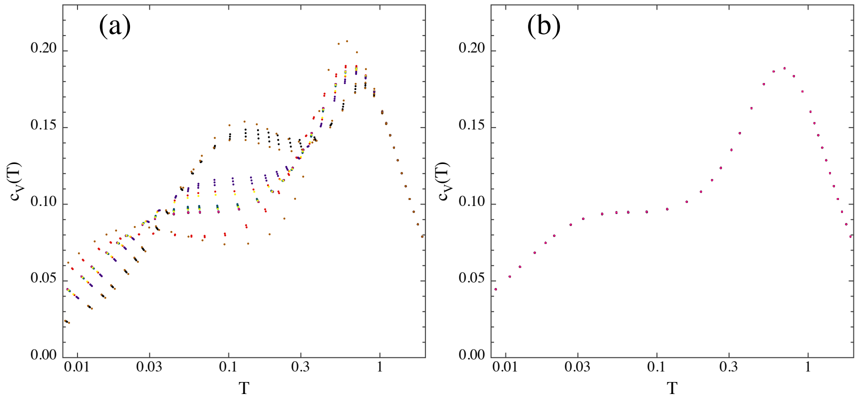


FIG. 13. (a) The 68 PAs of $c_V(T)$ from HTSE+$s(e)$found for orders 17-20, shown in the temperature range $[0.08, 1.5]$ for $\alpha = 1$, using $e_0 = -0.44$. The dots correspond to the energies at which the PAs are evaluated. If at the highest temperatures shown here, the dots are vertically aligned ($T(e)$ is the same for all PAs), this is no more true for $T < 1$. (b) The corresponding 38 CPAs when the maximum distance between PAs is $\Delta = 0.001$. The dots are now almost vertically aligned for all temperatures.

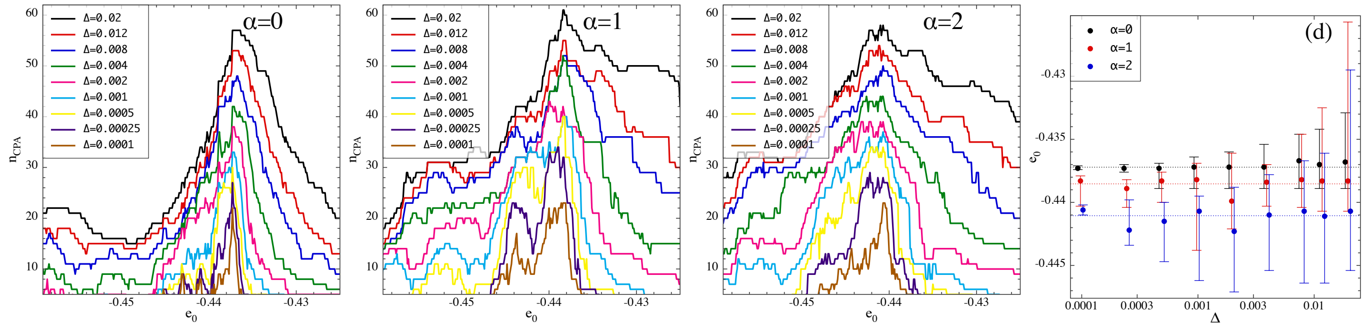


FIG. 14. (a)(b)(c) Number of CPAs found for $c_V(T)$ HTSE+$s(e)$versus the ground-state energy $e_0$ for different value of $\Delta$ for $\alpha = 0$, 1 and 2. (d) Best energy versus $\Delta$. At fixed $\Delta$, the error bars are obtained using the width of $n_{\text{CPA}}(e_0)$ evaluated at 0.8 of its maximum. The horizontal black (resp. red and blue) dashed line is the mean value through the data at $\alpha = 0$) (resp. 1 and 2).

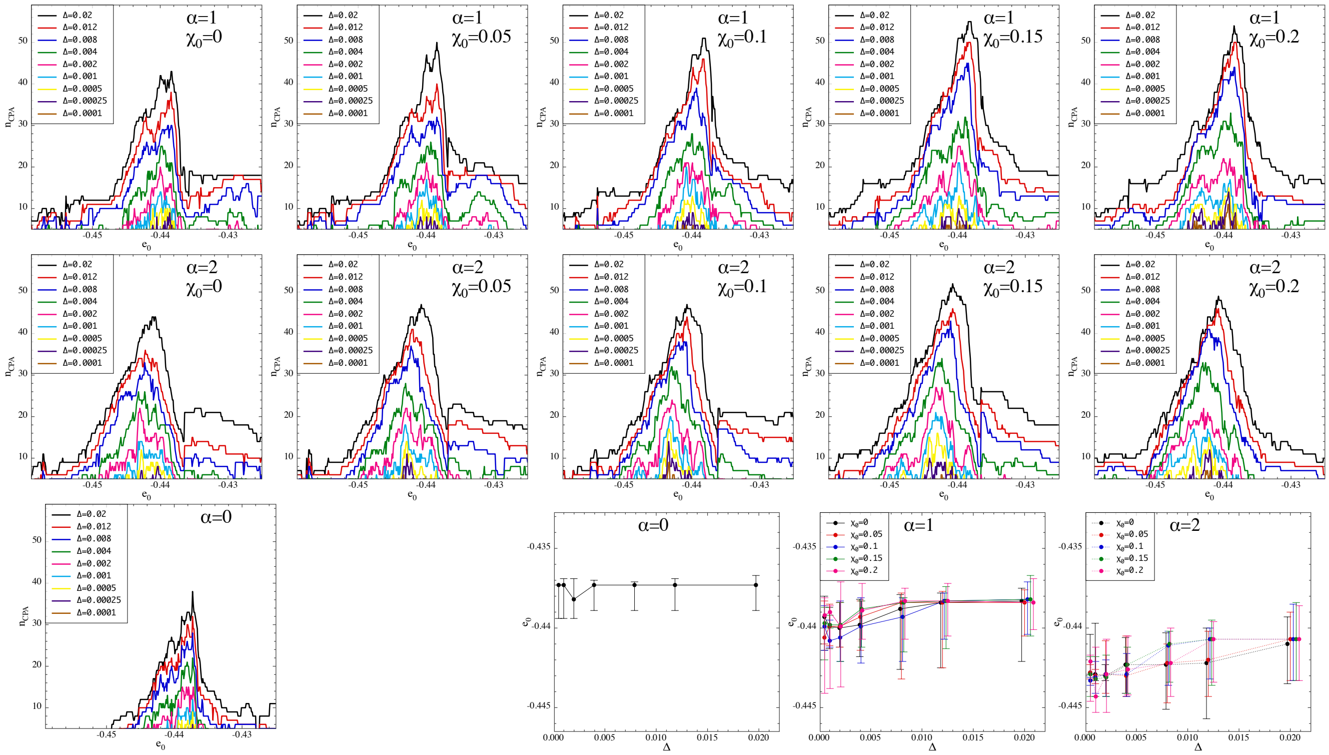


FIG. 15. Number of CPAs found for $\chi(T)$ versus the ground-state energy $e_0$ with various $\Delta$, the maximum distance between CPAs, for $\alpha = 1$ (first raw), 2 (second raw) and 0 (first figure of third raw) and $\chi_0$ as indicated on each plot. The three last figures compares the variations of the $e_0$ versus $\Delta$ for various $\chi_0$.

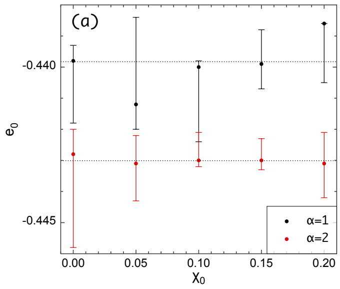


FIG. 16. Ground state energy versus $\chi_0$ from the CPAs of $\chi(T)$ for $\Delta = 0.001$. Constant horizontal lines are mean square fits.

## III. ATTEMPT FOR A DETERMINATION OF $\chi_0$

Eq. (32), $e_0(h) = e_0 - \chi_0\, h^2/2 + \mathcal{O}(h^4)$, relates $\chi_0$, the magnetic susceptibility at $T = 0$, with the second derivative of the ground state energy with respect to the magnetic field. We propose here to use our protocole defined in Sec. II F to evaluate $e_0(h)$ and deduce $\chi_0$. We first determine $\chi_0$ for the KHAF and then its variations when adding perturbations.

### A. KHAF

Fig. 17 shows the influence of the magnetic field $h$ on the specific heat $c_V$ when $e_0$ is determined with the protocole defined in Sec. II F. Fig. 17-d shows how $e_0$ varies with $h$. The vertical error bars indicate the uncertainties in the determinations of $e_0$. The lines are linear fit in $h^2$ through all points. This leads to values of $\chi_0$ around 0.22, 0.28 and 0.36 for $\alpha = 0$, 1 and 2 respectively. But clearly, an horizontal line can go through all points with $h \lesssim 0.05$. For the gapped case, we expect to find $\chi_0 = 0$ at least at small $h$. Indeed, $\chi_0 = 0$ is not incompatible with our data for $h < 0.07$. Thus this method gives an upper bound for $\chi_0$ around 0.3, in agreement with the PAs of $\chi(e)$ (see Figs. 11 and 12-c-d).

In the following sections we look for effects of various perturbations on such evaluation of $\chi_0$.

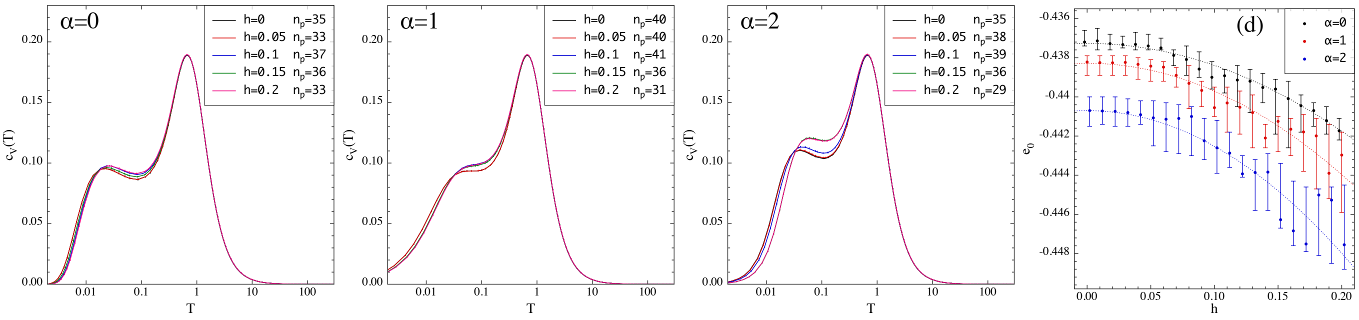


FIG. 17. $\alpha = 0$, 1 and 2: Influence of the magnetic field $h$ on the specific heat, $c_V$, when $e_0(h)$ is found using the protocole of Sec. II F for $\alpha = 0$, 1 and 2. (d) Evolution of $e_0$ with $h$ using this protocole.

### B. Influence of impurities

Fig. 18 shows the influence of impurities, $p$, when $e_0$ is determined with the protocole defined in Sec. II F. Tab. I gives the values of $\chi_0$, evaluated from a linear fit in $h^2$ through all points, that decrease when $p$ increases. Note that a smaller curvature ($\chi_0$) is compatible with the first points.

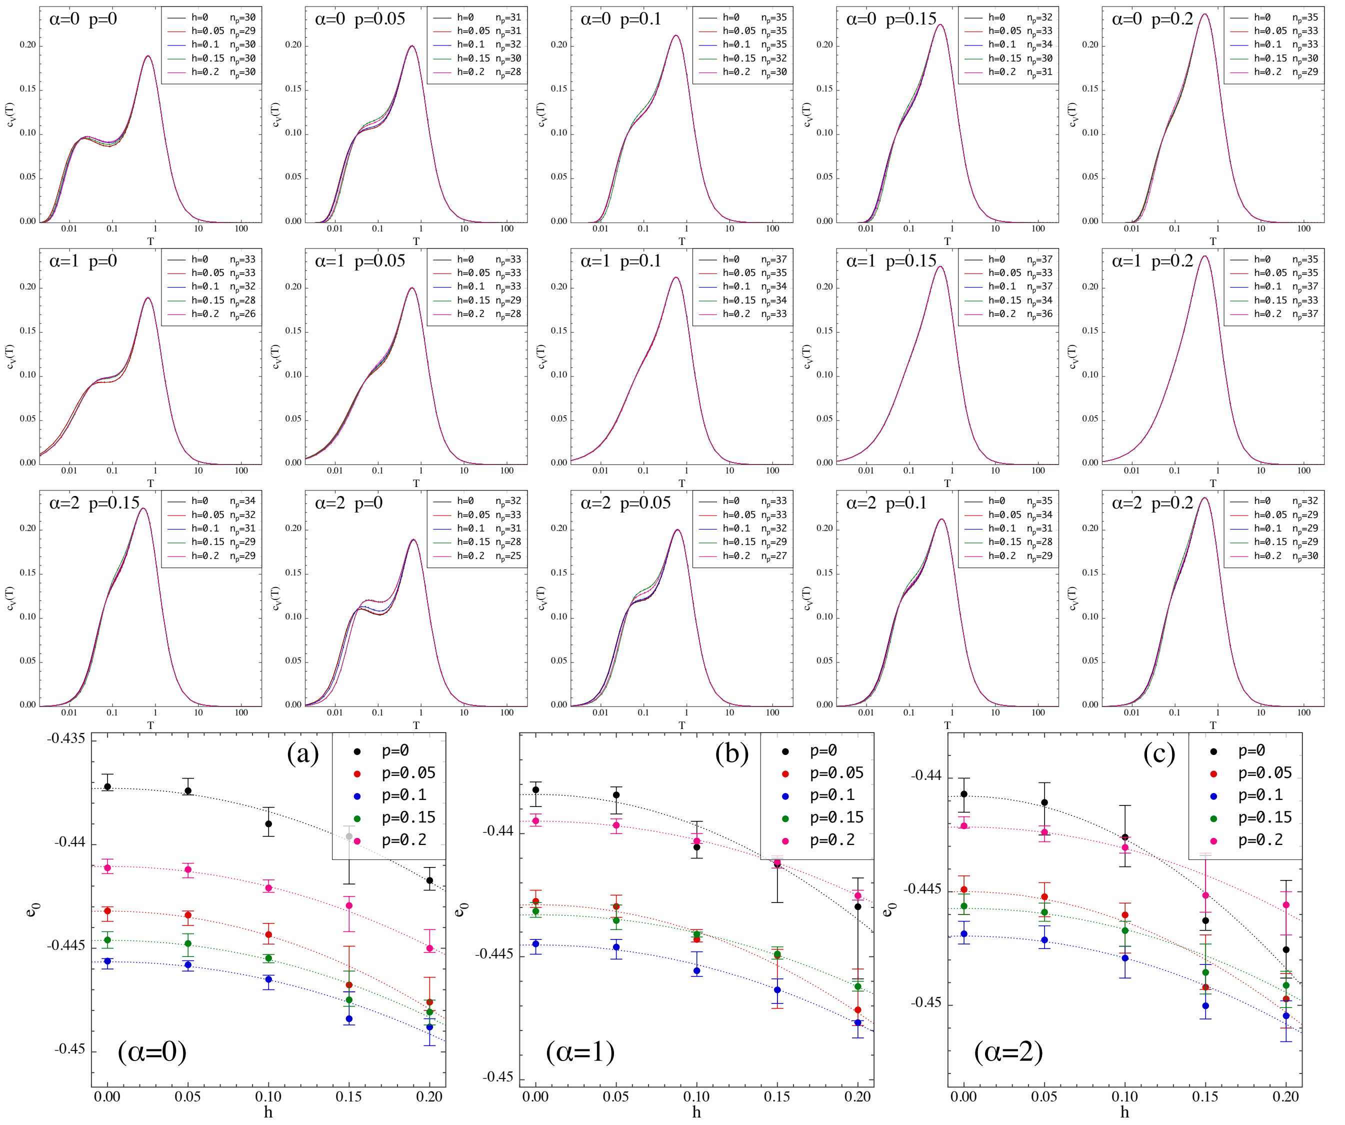


FIG. 18. Influence of the magnetic field $h$ on the specific heat $c_V$ for various impurities ratios $p$.

| $p$ | 0 | 0.05 | 0.10 | 0.15 | 0.20 |
|---|---|---|---|---|---|
| $\alpha$ =0 | 0.23 | 0.24 | 0.17 | 0.19 | 0.19 |
| $\alpha$ =1 | 0.25 | 0.22 | 0.16 | 0.15 | 0.15 |
| $\alpha$ =2 | 0.38 | 0.27 | 0.19 | 0.19 | 0.19 |

TABLE I. Variations of $\chi_0$ with $p$, from linear fits in $h^2$ of the data of Fig.18 (see dotted lines of Fig.18-a-b-c).

### C. Influence of Dzyaloshinskii–Moriya interaction

Fig. 19 shows the influence of a Dzyaloshinskii–Moriya interaction, $D_z$, when $e_0$ is determined with the protocole defined in Sec. II F. Tab. II gives the values of $\chi_0$, evaluated from a linear fit in $h^2$ through all points, that decreases when $D_z$ increases. Note that a smaller curvature ($\chi_0$) is compatible with the first points.

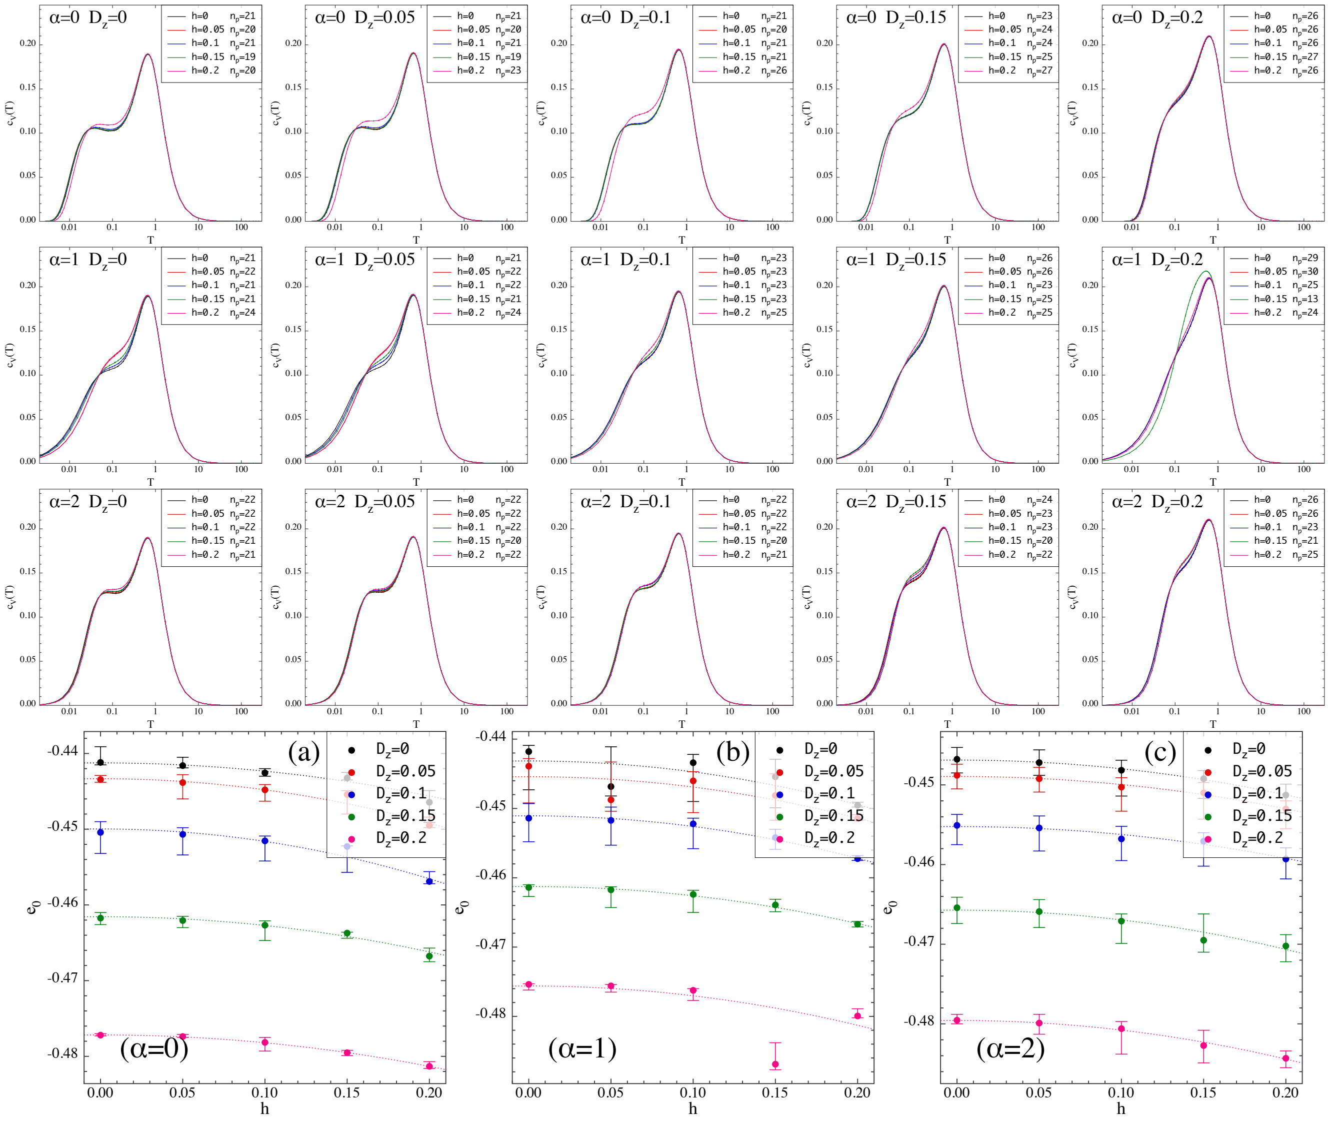

FIG. 19. Influence of the magnetic field $h$ on the specific heat $c_V$ for various DM interaction strengths $D_z$.

| $D_z$ | 0 | 0.05 | 0.10 | 0.15 | 0.20 |
|---|---|---|---|---|---|
| $\alpha$ =0 | 0.22 | 0.29 | 0.33 | 0.23 | 0.21 |
| $\alpha$ =1 | 0.32 | 0.30 | 0.31 | 0.27 | 0.28 |
| $\alpha$ =2 | 0.22 | 0.20 | 0.20 | 0.25 | 0.24 |

TABLE II. Variations of $\chi_0$ with $D_z$, from linear fits in $h^2$ of the data of Fig.19 (see dotted lines of Fig.19-a-b-c).

### D. Influence of an Ising interaction

Fig. 20 shows the influence of an additional Ising interaction, $\delta_z$, when $e_0$ is determined with the protocole defined in Sec. II F. Tab. III gives the values of $\chi_0$, evaluated from a linear fit in $h^2$ through all points.

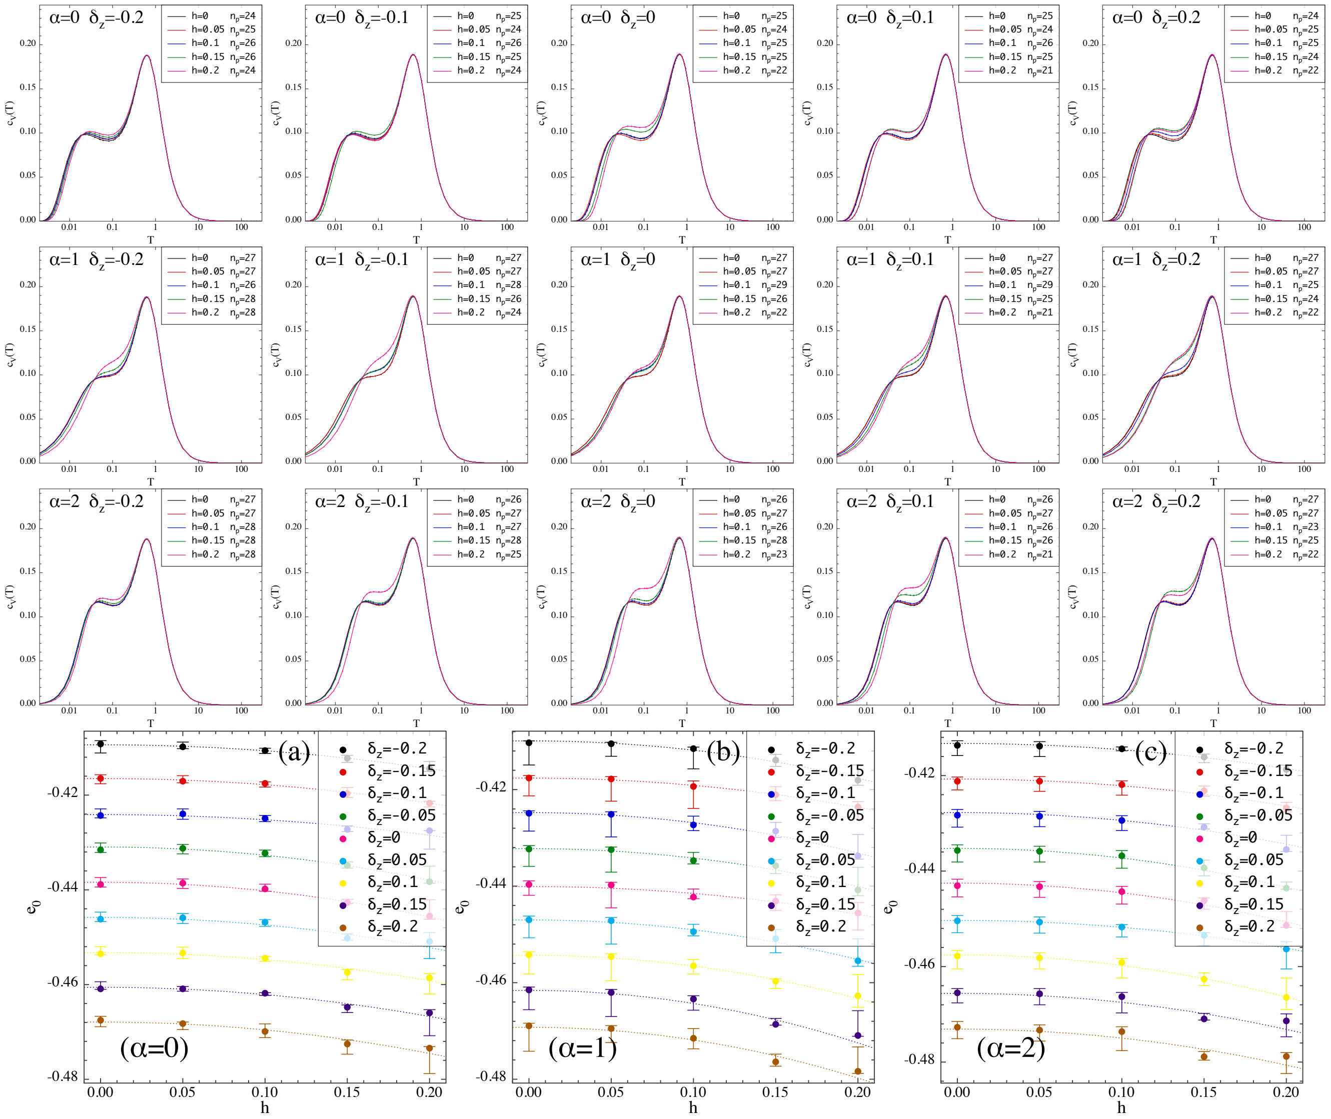


FIG. 20. Influence of the magnetic field $h$ on the specific heat $c_V$ for various values of the Ising interaction $\delta_z$.

| $\delta_z$ | -0.20 | -0.15 | 0.10 | -0.05 | 0 | 0.05 | 0.10 | 0.15 | 0.20 |
|---|---|---|---|---|---|---|---|---|---|
| $\alpha=0$ | 0.25 | 0.26 | 0.22 | 0.35 | 0.37 | 0.32 | 0.30 | 0.31 | 0.33 |
| $\alpha=1$ | 0.39 | 0.30 | 0.42 | 0.39 | 0.29 | 0.41 | 0.45 | 0.54 | 0.53 |
| $\alpha=2$ | 0.26 | 0.28 | 0.33 | 0.41 | 0.41 | 0.29 | 0.44 | 0.38 | 0.38 |

TABLE III. Variations of $\chi_0$ with $\delta_z$, from linear fits in $h^2$ of the data of Fig.20 (see dotted lines of Fig.20-a-b-c).

### E. Influence a second neighbor interaction $J_2$

Fig. 21 shows the influence of a second neighbor interaction, $J_2$, when $e_0$ is determined with the protocole defined in Sec. II F. Tab. IV gives the values of $\chi_0$, evaluated from a linear fit in $h^2$ through all points. Again here, a much smaller curvature ($\chi_0$) is compatible with the first points.

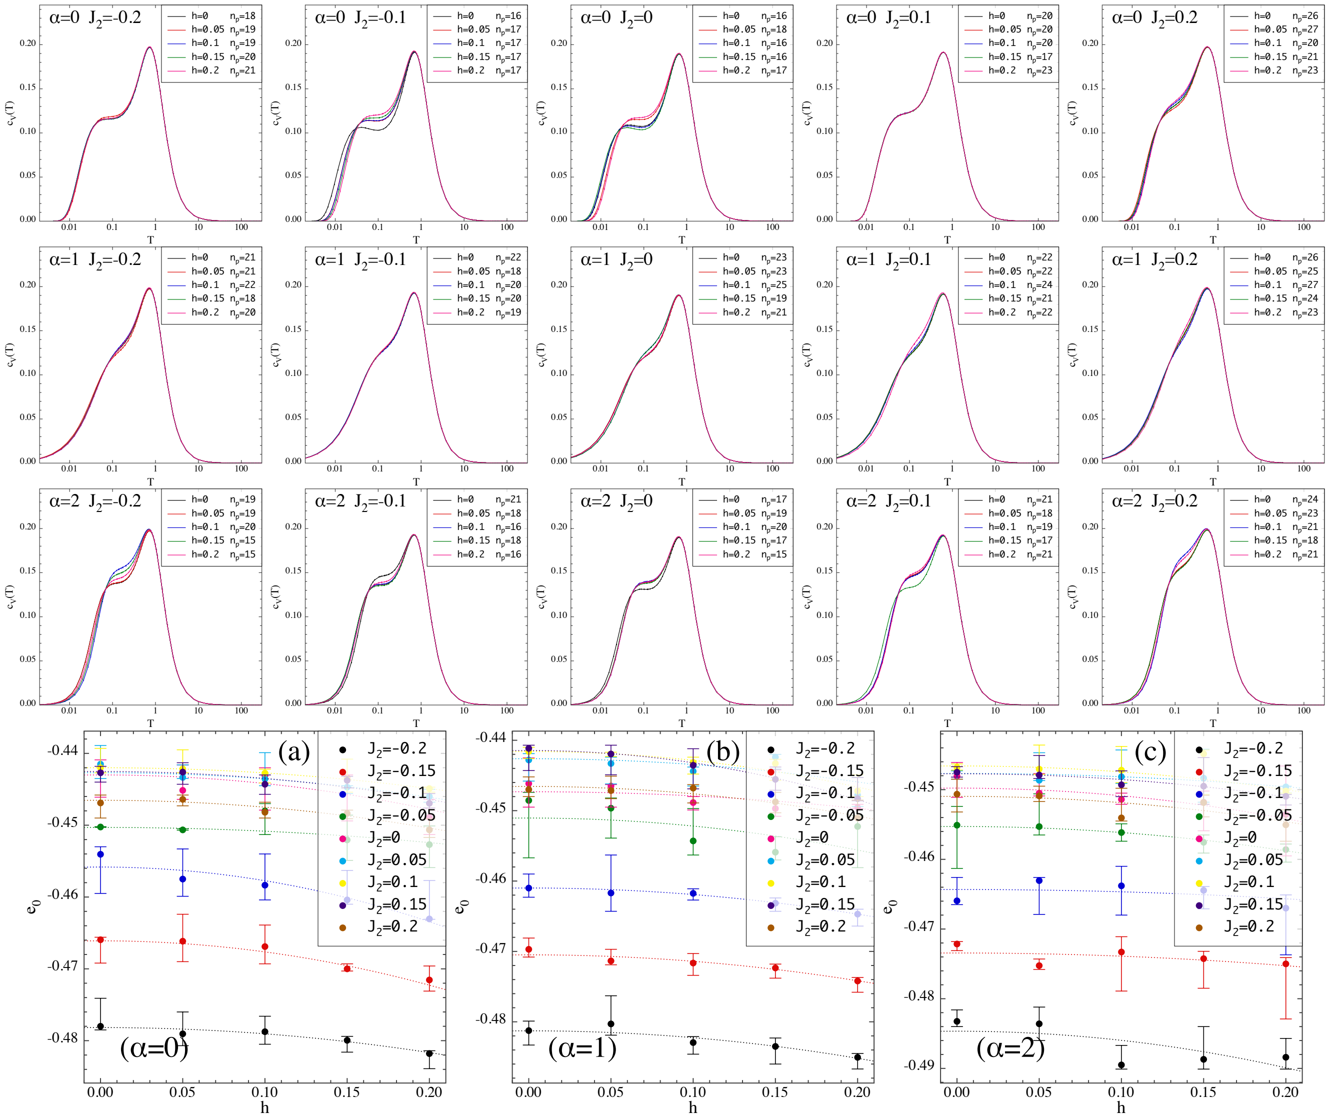


FIG. 21. Influence of the magnetic field $h$ on the specific heat $c_V$ for various values of $J_2$, the second neighbor interaction.

| $J_2$ | -0.20 | -0.15 | -0.10 | -0.05 | 0 | 0.05 | 0.10 | 0.15 | 0.20 |
|---|---|---|---|---|---|---|---|---|---|
| $\alpha=0$ | 0.17 | 0.31 | 0.38 | 0.11 | 0.24 | 0.17 | 0.15 | 0.20 | 0.19 |
| $\alpha=1$ | 0.20 | 0.18 | 0.19 | 0.23 | 0.12 | 0.17 | 0.25 | 0.30 | 0.21 |
| $\alpha=2$ | 0.27 | 0.09 | 0.07 | 0.17 | 0.22 | 0.10 | 0.17 | 0.17 | 0.18 |

TABLE IV. Values of $\chi_0$ from linear fits in $h^2$ of the data of Fig.21 (see dotted lines of Fig.21-a-b-c).

### F. Influence a third neighbor interaction $J_3$

Fig. 22 shows the influence of a third neighbor interaction, $J_3$, when $e_0$ is determined with the protocole defined in Sec. II F. Tab. V gives the values of $\chi_0$, evaluated from a linear fit in $h^2$ through all points. Again here, a much smaller curvature ($\chi_0$) is compatible with the first points.

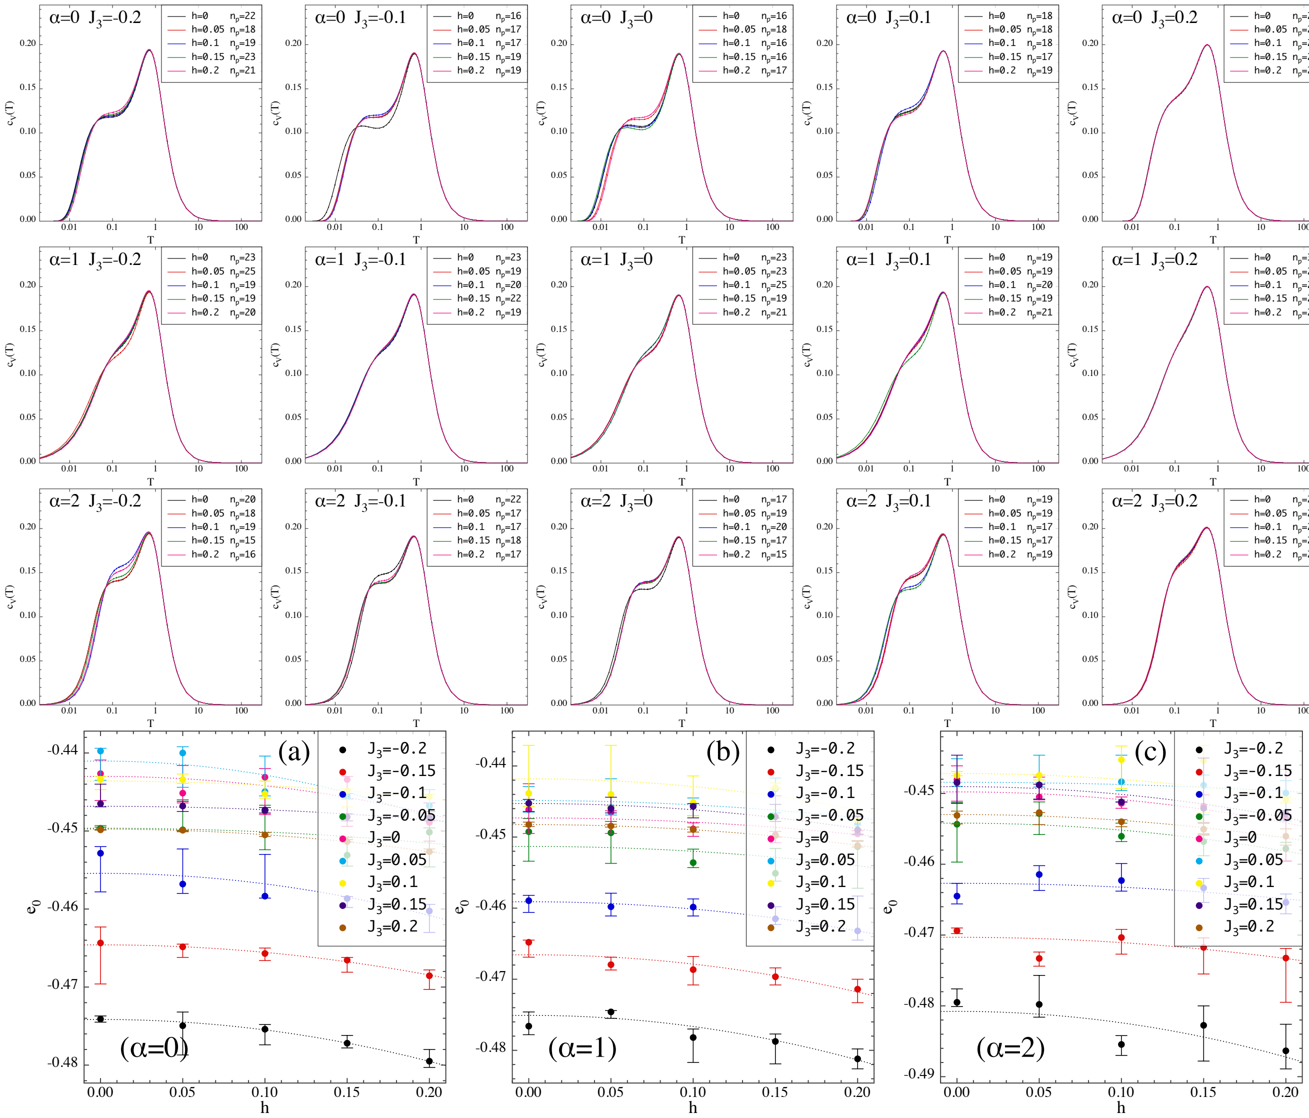


FIG. 22. Influence of the magnetic field $h$ on the specific heat $c_V$ for various values of $J_3$, the third neighbor interaction.

| $J_3$ | -0.20 | -0.15 | -0.10 | -0.05 | 0 | 0.05 | 0.10 | 0.15 | 0.20 |
|---|---|---|---|---|---|---|---|---|---|
| $\alpha=0$ | 0.27 | 0.19 | 0.27 | 0.10 | 0.24 | 0.36 | 0.11 | 0.09 | 0.14 |
| $\alpha=1$ | 0.31 | 0.26 | 0.21 | 0.14 | 0.12 | 0.12 | 0.22 | 0.18 | 0.15 |
| $\alpha=2$ | 0.32 | 0.15 | 0.11 | 0.20 | 0.22 | 0.06 | 0.17 | 0.22 | 0.17 |

TABLE V. Values of $\chi_0$ from linear fits in $h^2$ of the data of Fig.22 (see dotted lines of Fig.22-a-b-c).

### G. Influence a third neighbor interaction $J_{3h}$

Fig. 23 shows the influence of a third neighbor interaction, $J_{3h}$, when $e_0$ is determined with the protocole defined in Sec. II F. Tab. VI gives the values of $\chi_0$, evaluated from a linear fit in $h^2$ through all points. Again here, a much smaller curvature ($\chi_0$) is compatible with the first points.

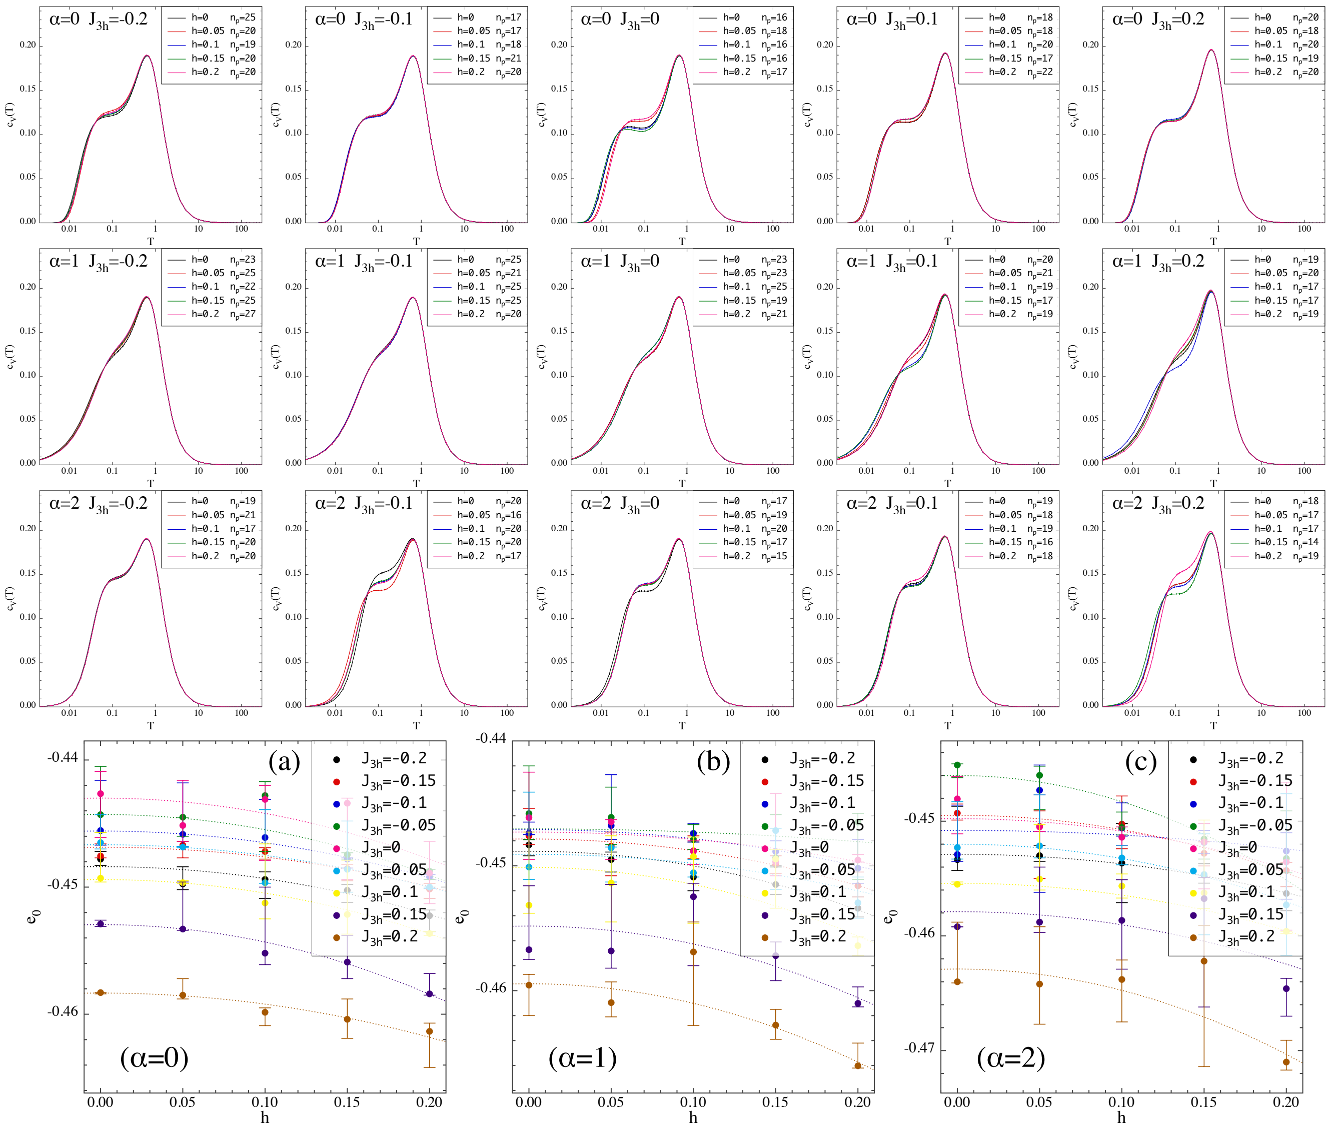


FIG. 23. Influence of the magnetic field $h$ on the specific heat $c_V$ for various values of $J_{3h}$, the third neighbor interaction.

| $J_{3h}$ | -0.20 | -0.15 | -0.10 | -0.05 | 0 | 0.05 | 0.10 | 0.15 | 0.20 |
|---|---|---|---|---|---|---|---|---|---|
| $\alpha=0$ | 0.19 | 0.16 | 0.19 | 0.24 | 0.24 | 0.17 | 0.21 | 0.27 | 0.17 |
| $\alpha=1$ | 0.24 | 0.19 | 0.15 | 0.05 | 0.12 | 0.15 | 0.28 | 0.29 | 0.31 |
| $\alpha=2$ | 0.17 | 0.25 | 0.08 | 0.46 | 0.22 | 0.25 | 0.21 | 0.23 | 0.37 |

TABLE VI. Values of $\chi_0$ from linear fits in $h^2$ of the data of Fig.23 (see dotted lines of Fig.23-a-b-c).

# IV. INFLUENCE OF PERTURBATIONS ON THE KHAF

## A. Influence of impurities

Let $p$ be the ratio of missing spins. Fig. 24 shows how $C_V(T)$ varies with $p$. The ground state energy (Fig. 24-(d)). is adjusted for each $p$ according to the protocole defined in II F. As expected, $e_0$ first decreases as $p$ increases from 0, but it reaches a minimum around $p = 0.1$ and then increases with $p$. A few percents of impurities has already a significant effect on the $c_V(T)$. The maximum of $c_V$ almost increases linearly with $p$, washing out the low-$T$ bump.

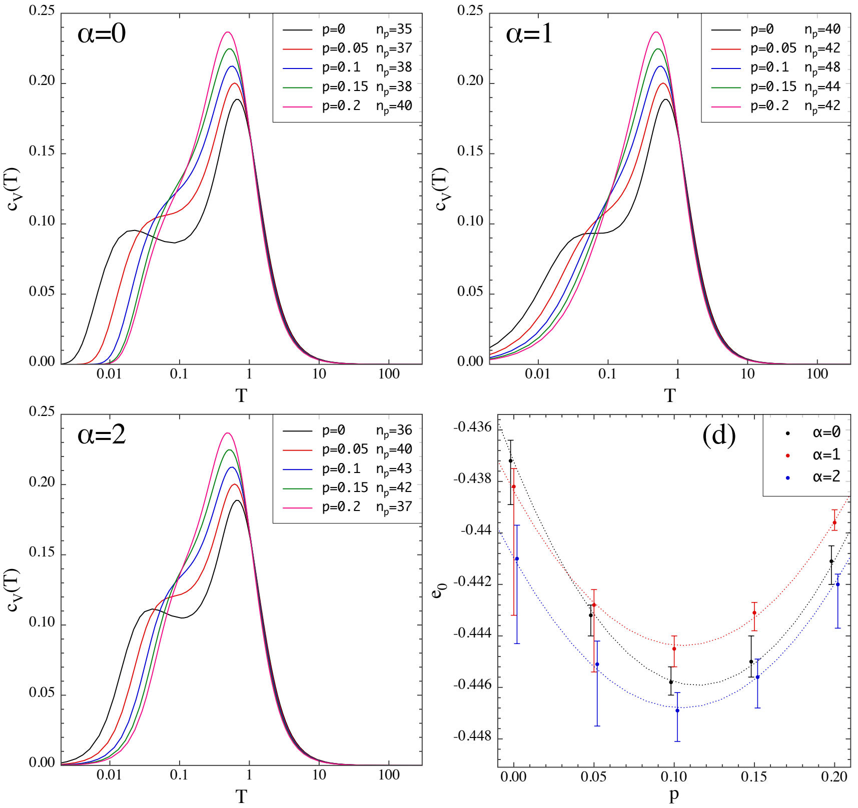


FIG. 24. Influence of the impurity ratio $p$ on the specific heat $c_V$ for $\alpha = 0$, 1 and 2. $n_p$ is the number of CPAs. (d) ground state energy $e_0$ (dots) versus $p$ for $\alpha = 0$, 1 and 2. Dotted lines are the quadratic fits: $-0.4372 - 0.1517\,p + 0.6627\,p^2$, $-0.4384 - 0.1107\,p + 0.5257\,p^2$ and $-0.4421 - 0.0907\,p + 0.4543\,p^2$ for $\alpha = 0$, 1 and 2 respectively.

Tab. VII shows the almost linear variations of the parameter $T_0$, as defined in Eqs.(27)-(30), with respect to $p$. For each value of $\alpha$, $T_0$ increases amost linearly with $p$ up to $p = 0.15$: $T_0 \simeq 0.0223 + 0.465\,p$ for $\alpha = 0$, $T_0 \simeq 0.172 + 2.4\,p$ for $\alpha = 1$ and $T_0 \simeq 0.0475 + 0.51\,p$ for $\alpha = 2$.

| $p$ | 0 | 0.05 | 0.1 | 0.15 | 0.2 |
|---|---|---|---|---|---|
| $\alpha = 0$ | 0.02236(14) | 0.04433(21) | 0.0707(6) | 0.091(9) | 0.0958(7) |
| $\alpha = 1$ | 0.1703(11) | 0.2895(13) | 0.4239(21) | 0.529(20) | 0.623(3) |
| $\alpha = 2$ | 0.04724(27) | 0.07239(30) | 0.1015(4) | 0.1233(5) | 0.1397(5) |

TABLE VII. Dependency of $T_0$, as defined in Eqs.(27)-(30) with respect to $p$.

For $\chi$, we use the $e_0(p)$ found for $c_V$, independently of the value of $\chi_0$. Fig. 25 and 26 shows the influence of $p$ and $\chi_0$ for $\alpha = 0$, 1 and 2. $\chi(T)$ is almost insensitive to $\alpha$. Below $T < 0.01$, $\chi(T) \sim \chi_0$, thus independent of $p$ or $\alpha$. For $T > 0.4$, $\chi(T)$ is independent of $\chi_0$ and $\alpha$. Nevertheless, the number of CPAs is slightly larger for $\alpha = 1$.

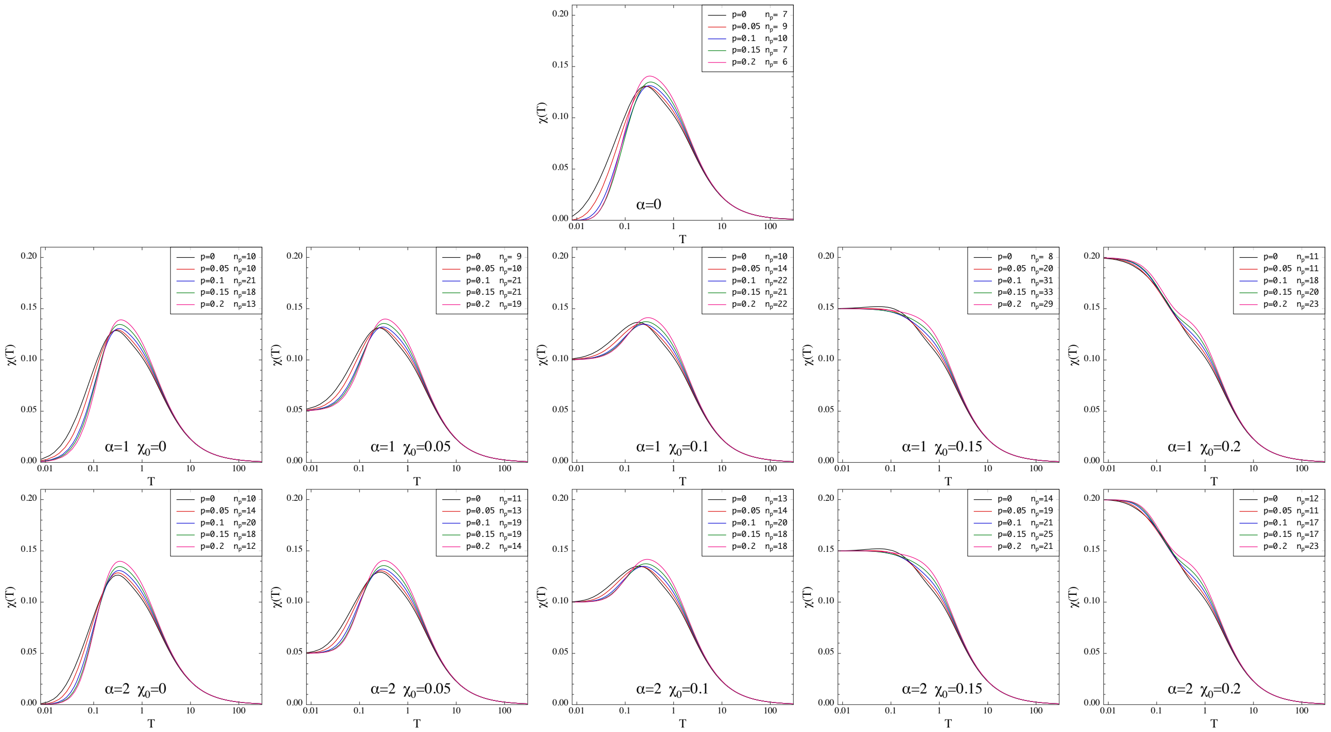


FIG. 25. Influence of the impurity ratio $p$ on the magnetic susceptibility $\chi(T)$ for $\alpha = 0$, 1 and 2 and for various values of $\chi_0$ within HTSE+$s(e)$. $n_p$ is the number of CPAs.

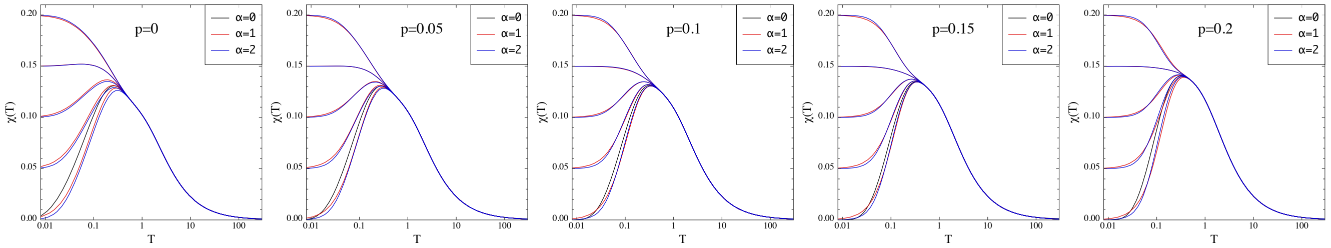


FIG. 26. Influence of $\chi_0$ on the magnetic susceptibility $\chi$ for various impurity ratios $p$ within HTSE+$s(e)$. Same data as Fig. 25, but at $p$ constant.

### B. Influence of the magnetic field

We show here the influence of the magnetic field $h$ on the specific heat $c_V$ and the magnetic susceptibility $\chi$. The applied magnetic fields are $h = 0.05$, 0.1, 0.15 and 0.2. $e_0$ varies with $h$ as defined in Eq. (32). We use the best ground state energy found in Sec. II F: $e_0 = -04372$ for $\alpha = 0$, $e_0 = -04391$ for $\alpha = 1$ and -0.4417 for $\alpha = 2$. Thus when $h \neq 0$, $c_V(T)$ depends on $e_0$ and on $\chi_0$ for a fixed $\alpha$.

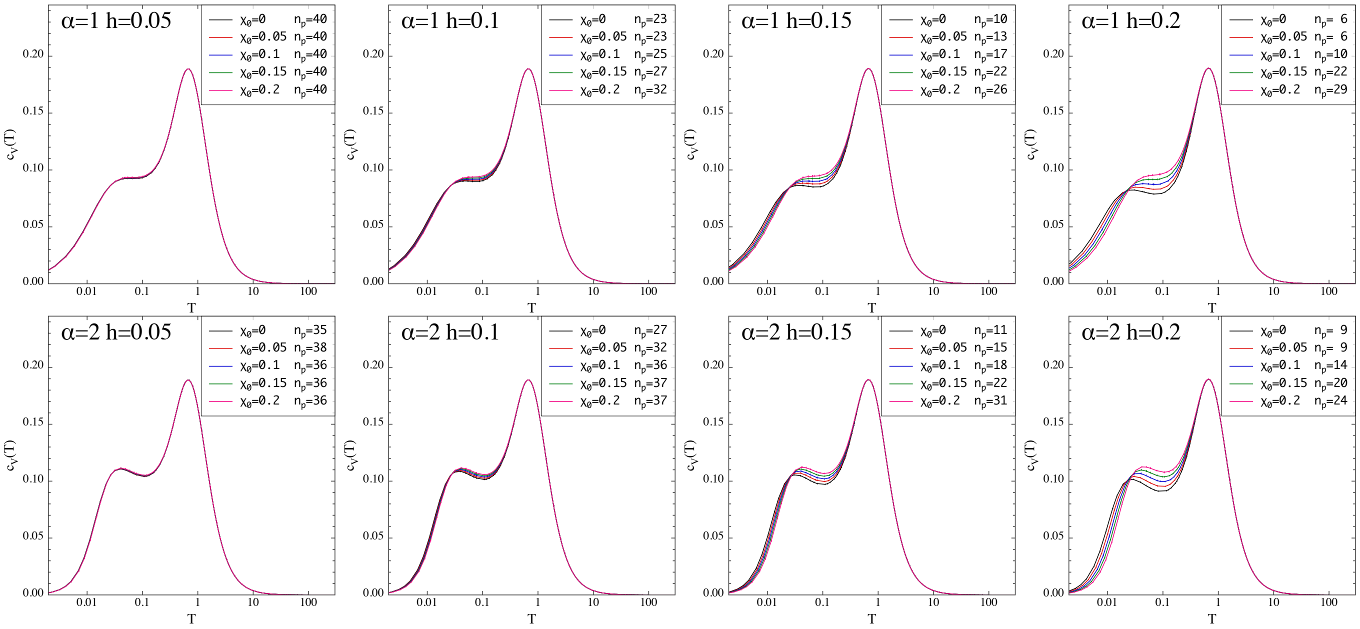


FIG. 27. Influence of the magnetic field $h$ on $c_V(T)$ for $\alpha = 1$ (first raw) and 2 (second raw) within HTSE+$s(e)$. Each figure is at fixed $h$. $n_p$ indicates the number of CPAs. Each figure is at a given magnetic field $h$ and for different $\chi_0$.

At $h = 0$, $e_0$ is independent of $\chi_0$. Fig. 27 shows how $c_V(T)$ varies at fixed $h \neq 0$ when $\chi_0$ varies. Above $T = 1$, $c_V(T)$, is insensitive to such low magnetic field. Below $h = 0.1$, the effects of $h$ are negligible. For $h > 0.1$, the effects increase with $\chi_0$, specially for temperatures around 0.1. Fig. 28 shows how $c_V(T)$ varies at fixed $\chi_0$ when $h$ varies: $c_V(T \sim 0.1)$ decreases (resp. increases) when $h$ increases if $\chi_0 < 0.1$ (resp. $\chi_0 > 0.1$), while at $\chi_0 = 0.1$, $h$ has almost no effect.

Tab. VIII shows the parameter $T_0$ as defined in Eqs.(27)-(30). For each $\alpha$, $T_0$ decreases with $h$ and for $\alpha > 0$ increases with $\chi_0$.

| | $h$ | 0 | 0.05 | 0.1 | 0.15 | 0.2 |
|---|---|---|---|---|---|---|
| $\alpha = 0$ | $\chi_0 = 0$ | 0.02236(14) | 0.0217(17) | 0.01974(19) | 0.01632(12) | 0.01357(13) |
| $\alpha = 1$ | $\chi_0 = 0$ | 0.1703(11) | 0.167(14) | 0.1564(11) | 0.1375(10) | 0.1159(7) |
| | $\chi_0 = 0.05$ | 0.1703(11) | 0.1681(13) | 0.1605(9) | 0.1481(13) | 0.1311(4) |
| | $\chi_0 = 0.1$ | 0.1703(11) | 0.1691(12) | 0.1644(11) | 0.1577(11) | 0.1479(11) |
| | $\chi_0 = 0.15$ | 0.1703(11) | 0.1701(12) | 0.169(11) | 0.1681(10) | 0.1666(13) |
| | $\chi_0 = 0.2$ | 0.1703(11) | 0.1711(11) | 0.1737(12) | 0.1785(15) | 0.1849(14) |
| $\alpha = 2$ | $\chi_0 = 0$ | 0.04724(27) | 0.04643(20) | 0.04382(16) | 0.0398(19) | 0.03447(18) |
| | $\chi_0 = 0.05$ | 0.04724(27) | 0.0468(24) | 0.04491(22) | 0.0423(29) | 0.03825(13) |
| | $\chi_0 = 0.1$ | 0.04724(27) | 0.04704(25) | 0.04611(25) | 0.04469(18) | 0.0425(25) |
| | $\chi_0 = 0.15$ | 0.04724(27) | 0.04728(24) | 0.04712(25) | 0.04695(20) | 0.04655(25) |
| | $\chi_0 = 0.2$ | 0.04724(27) | 0.04752(24) | 0.04808(22) | 0.04947(24) | 0.05075(20) |

TABLE VIII. Dependency of $T_0$ with respect to $h$.

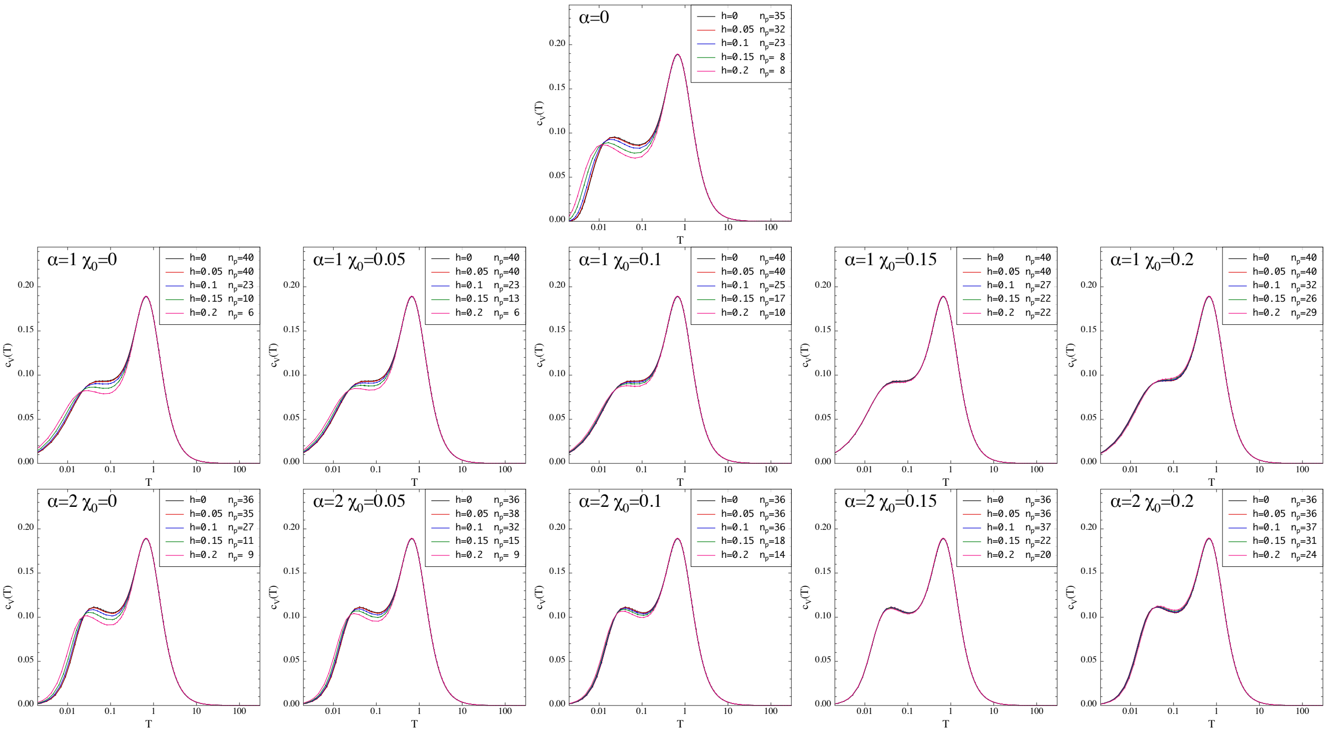


FIG. 28. Influence of the magnetic field on $c_V(T)$ for $\alpha = 0$ (first raw), $\alpha = 1$ (second raw) and $\alpha = 2$ (last raw) within HTSE+$s(e)$. Same data as Fig. 27 but at fixed $\chi_0$.

Fig. 30 shows how $\chi(T)$ varies at fixed $h$ when $\chi_0$ varies ($\alpha \neq 0$). At low temperature ($T < 0.01$), $\chi(T)$ is dominated by the imposed value $\chi_0$, here independent of $h$, while the high temperature ($T > 1$) is given by the HTSE which appear to be insensitive to these *low* $h$. As $h$ increases the number of CPAs decreases at small $\chi_0$, while it is almost constant at $\chi_0 = 0.2$. Fig. 29 shows that $\chi(T)$ is almost insensitive to $h$ at all temperature.

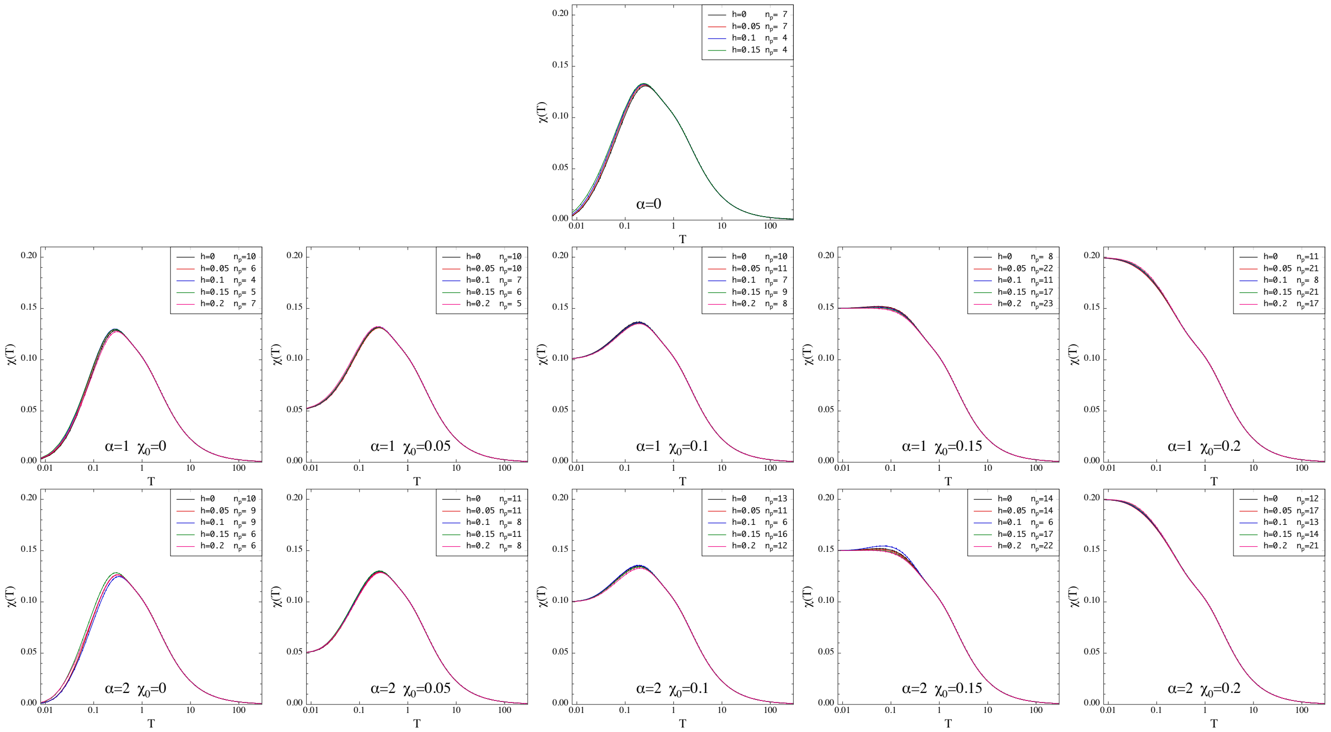


FIG. 29. Influence of the magnetic field $h$ on $\chi(T)$, at fixed $\chi_0$ for $\alpha = 0$ (first raw), $\alpha = 1$ (second raw) and $\alpha = 2$ (last raw).

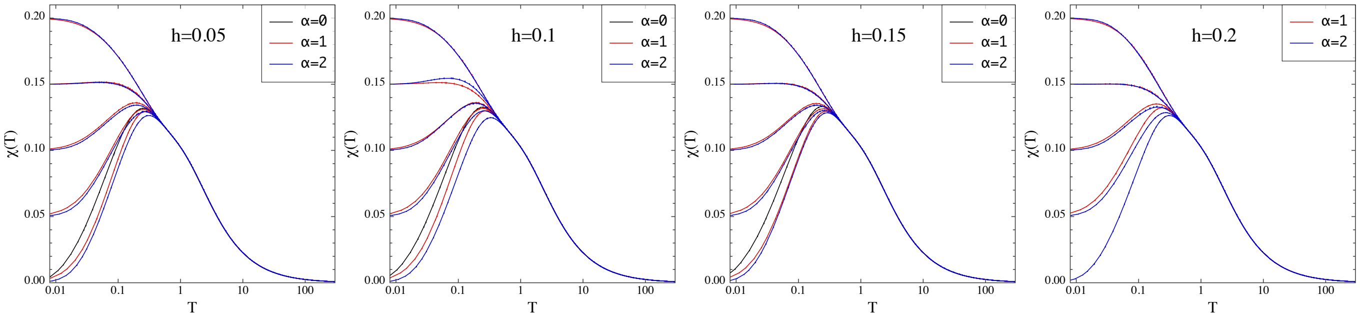


FIG. 30. Influence of the magnetic field $h$ on $\chi(T)$ (same data as Fig. 29 plotted at fixed $h$)

### C. Influence of Dzyaloshinskii–Moriya interaction

An out-of-plane Dzyaloshinskii–Moriya interaction (DMI) is added:

$$\mathcal{H}_{\rm DM} = \sum_{\langle i,j \rangle} D_z (S_i \wedge S_j)_z \tag{33}$$

The HTSE of $\frac{1}{N}\ln Z$ is obtained at order 16 in $\beta$ (same data as in Sec. I D).

The ground state energy $e_0$ varies with $D_z$. It has been adjusted on $c_V(T)$ according to the protocole of Sec. II F. Here we look at CPAs of HTSE from orders 13 to 16. Fig. 31-(a)-(c) shows that $D_z < 0.1$ has almost no effect on $c_V(T)$. $D_z \geq 0.1$ enhances the maximum of $c_V(T)$ and washes out the low-$T$ shoulder. Fig. 31-(d) shows the variations of $e_0$ with $D_z$, and the dotted lines are quadratic fits: $e_0 = -0.4413 - 0.8988\, D_z^2$ for $\alpha = 0$, $e_0 = -0.4422 - 0.8225\, D_z^2$ for $\alpha = 1$ and $e_0 = -0.4466 - 0.8184\, D_z^2$ for $\alpha = 2$.

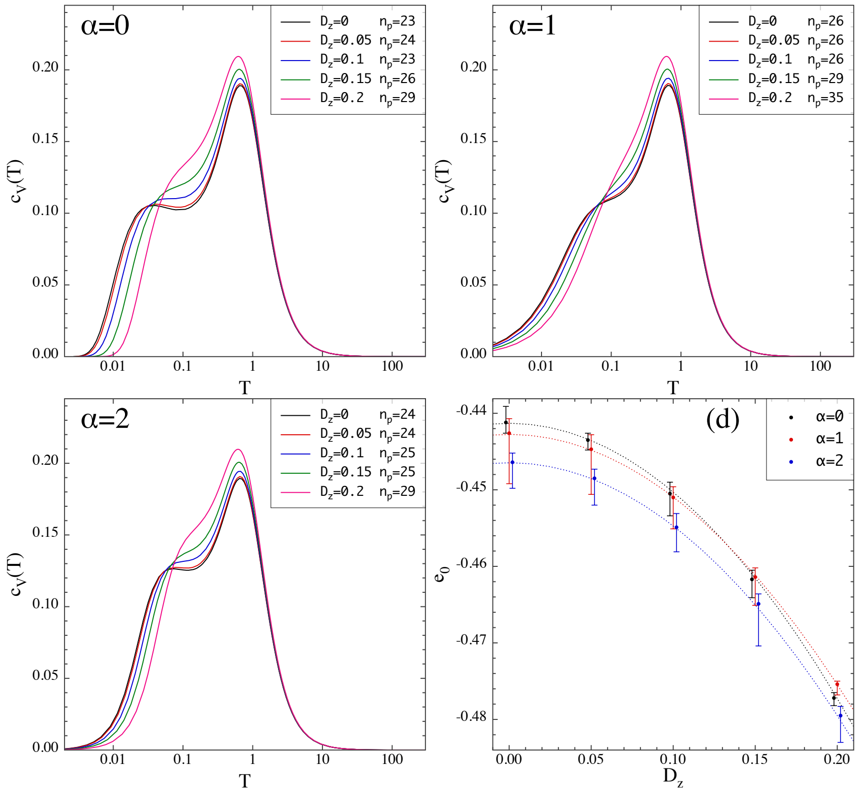


FIG. 31. (a)(b)(c) Influence of a Dzyaloshinskii–Moriya interaction $D_z$ on $c_V(T)$ for $\alpha = 0$, 1 and 2. (d) Ground state energy $e_0$ versus $D_z$ for $\alpha = 0$ (black), 1 (red) and 2 (blue). The dotted lines are quadratic fits.

Tab. IX shows the variations of the parameter $T_0$, as defined in Eqs.(27)-(30), with respect to $D_z$. For the three values of $\alpha$, $T_0$ roughly increases quadratically with $D_z$: $T_0 = 0.033 + 1.38\, D_z^2$ for $\alpha = 0$, $T_0 = 0.24 + 5.9\, D_z^2$ for $\alpha = 1$ and $T_0 = 0.068 + 1.4\, D_z^2$ for $\alpha = 2$.

| $D_z$ | 0 | 0.05 | 0.1 | 0.15 | 0.2 |
|---|---|---|---|---|---|
| $\alpha = 0$ | 0.03494(18) | 0.03719(23) | 0.04533(30) | 0.0606(4) | 0.0905(4) |
| $\alpha = 1$ | 0.2463(14) | 0.2574(13) | 0.2944(10) | 0.3666(18) | 0.4831(27) |
| $\alpha = 2$ | 0.06966(22) | 0.07237(21) | 0.08177(28) | 0.09666(29) | 0.1268(5) |

TABLE IX. Dependency of $T_0$ with respect to $D_z$.

Fig. 32 shows the effect of a DMI on the magnetic susceptibility. The ground state energy is the one found for $c_V(T)$ (Fig. 31-(d)). The effect of the DMI is negligible if $D \leq 0.15$, and small at $D = 0.2$.

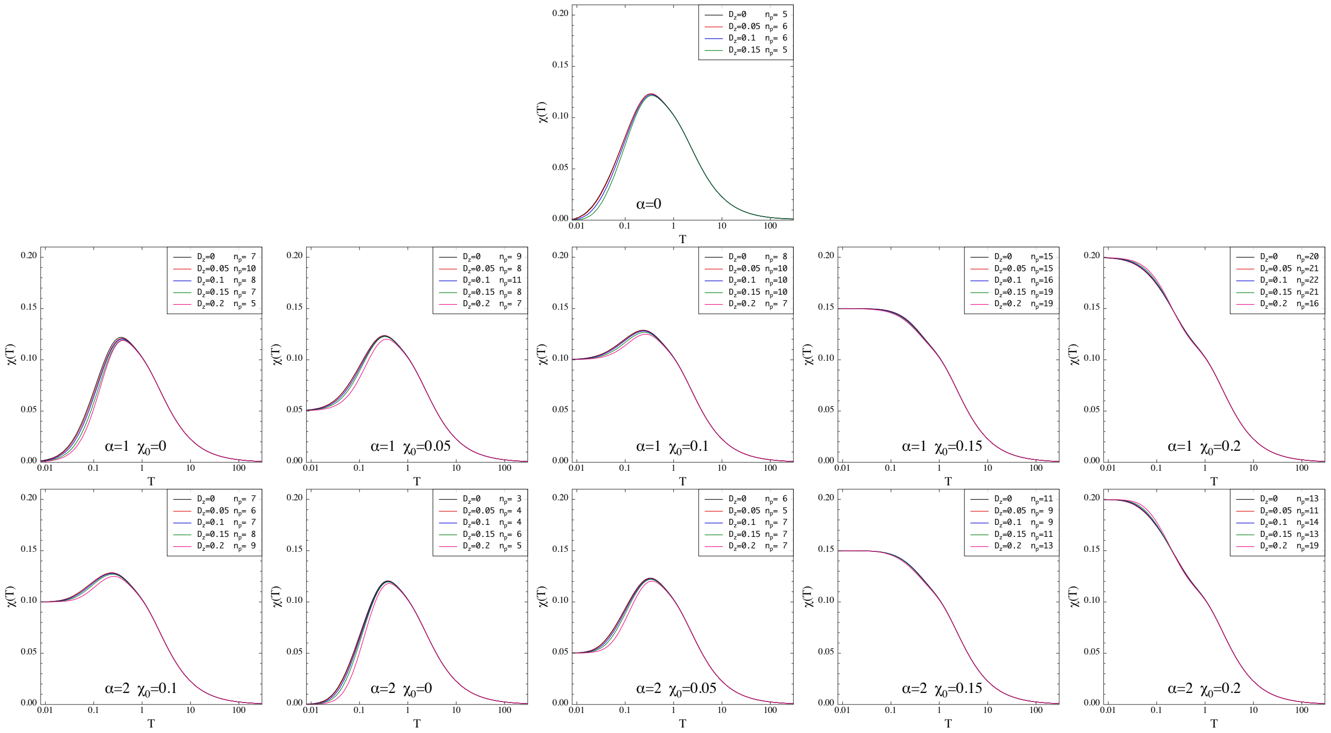


FIG. 32. Influence of Dzyaloshinskii–Moriya interaction $D_z$ on $\chi(T)$ for $\alpha = 0$ (first raw), $\alpha = 1$ (second raw) and $\alpha = 2$ (last raw).

Fig. 33 shows that $\alpha$ has almost no influence on $\chi(T)$.

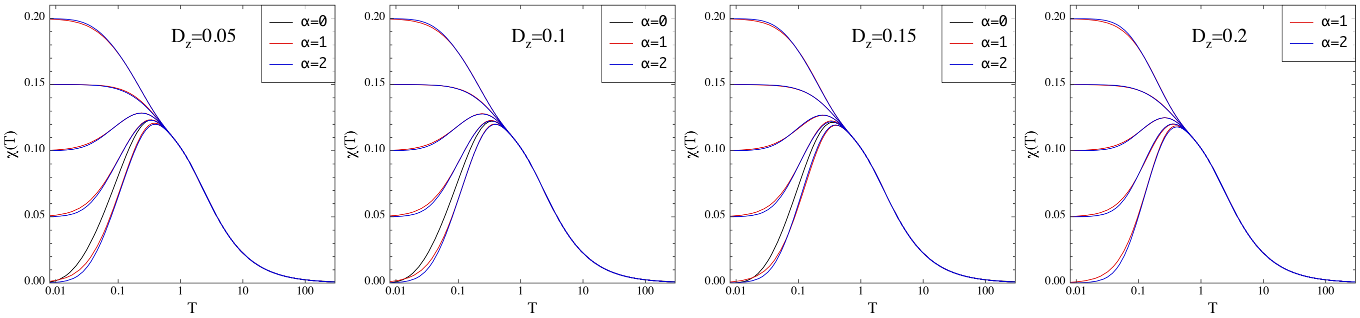


FIG. 33. Influence of Dzyaloshinskii–Moriya interaction $D_z$ on $\chi(T)$ (same data as Fig. 32, but plotted at fixed $D_z$).

### D. Influence of the Ising anisotropy

An Ising interaction, $\delta_z$, is added along the $z$ direction on each link ($XXZ$ model, see Eq. (10)). $\delta_z$ is varied from -0.2 to 0.2. The HT-series of $\frac{1}{N}\ln Z$ is obtained at order 18 in $\beta$ (same data as in Sec. I E). Here we look at CPAs for $\beta$-orders from 14 to 18.

The ground state energy $e_0$, adjusted on $c_V(T)$ according to the protocole of Sec.II F, varies linearly with $\delta_z$ (see Fig. 34-(c)). Fig. 34 shows that $\delta_z$ has almost no effect on the specific heat.

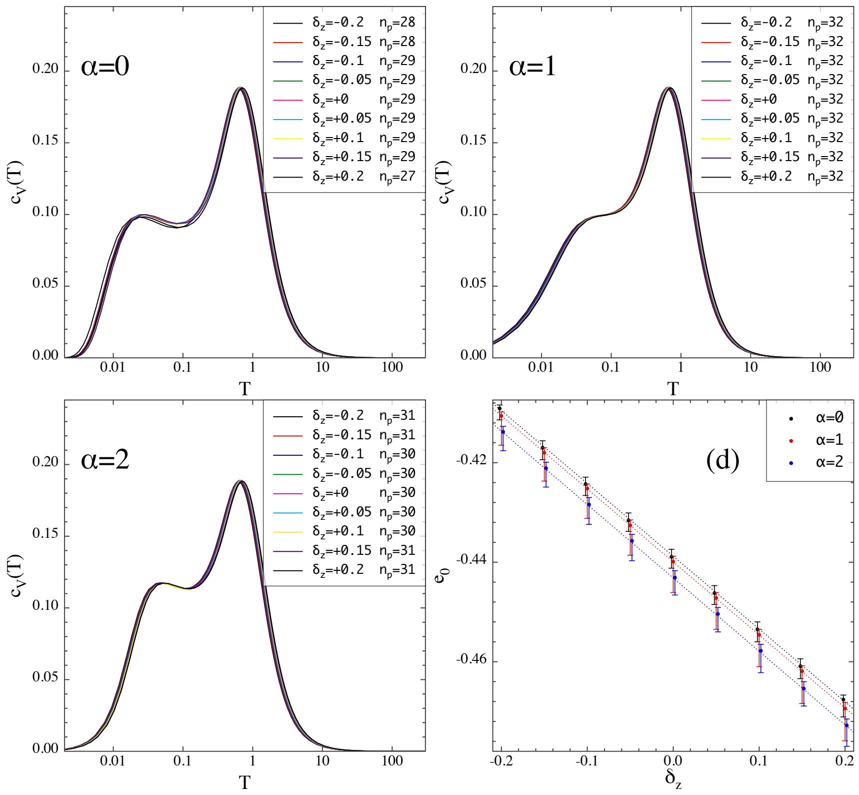

FIG. 34. (a)-(b)-(c) Influence of an Ising anisotropy $\delta_z$ on $c_V(T)$ for $\alpha = 0$, 1 and 2. (d) Ground state energy $e_0$ versus $\delta_z$ for $\alpha = 0$ (black), 1 (red) and 2 (blue); dotted lines are linear fits with a slope -0.147(1) in all cases.

Tab.X shows the variations of the parameter $T_0$, as defined in Eqs.(27)-(30), with respect to $\delta_z$. For the three values of $\alpha$, $T_0$ is roughly independent of $\delta_z$.

| $\delta_z$ | -0.2 | -0.15 | -0.1 | -0.05 | 0 | 0.05 | 0.1 | 0.15 | 0.2 |
|---|---|---|---|---|---|---|---|---|---|
| $\alpha = 0$ | 0.02719(23) | 0.02665(23) | 0.026(21) | 0.02352(17) | 0.02765(23) | 0.02802(24) | 0.02835(24) | 0.02886(26) | 0.02723(19) |
| $\alpha = 1$ | 0.1958(12) | 0.1907(13) | 0.188(12) | 0.1817(13) | 0.1989(12) | 0.2016(13) | 0.2051(13) | 0.2068(14) | 0.2115(14) |
| $\alpha = 2$ | 0.05474(26) | 0.05395(25) | 0.05307(27) | 0.052(28) | 0.0558(26) | 0.05632(28) | 0.05713(29) | 0.0587(3) | 0.0593(3) |

TABLE X. Dependency of $T_0$ with respect to $\delta_z$.

Fig. 35 shows the effect of $\delta_z$ on the magnetic susceptibility $\chi$. The ground state energy is the one found for $c_V(T)$ (Fig. 34-d). The effect of this anisotropy is to increase (resp. decrease) the magnetic susceptibility in the temperature range $[0.1 \ldots 1]$ when $\delta_z$ is negative (resp. positive).

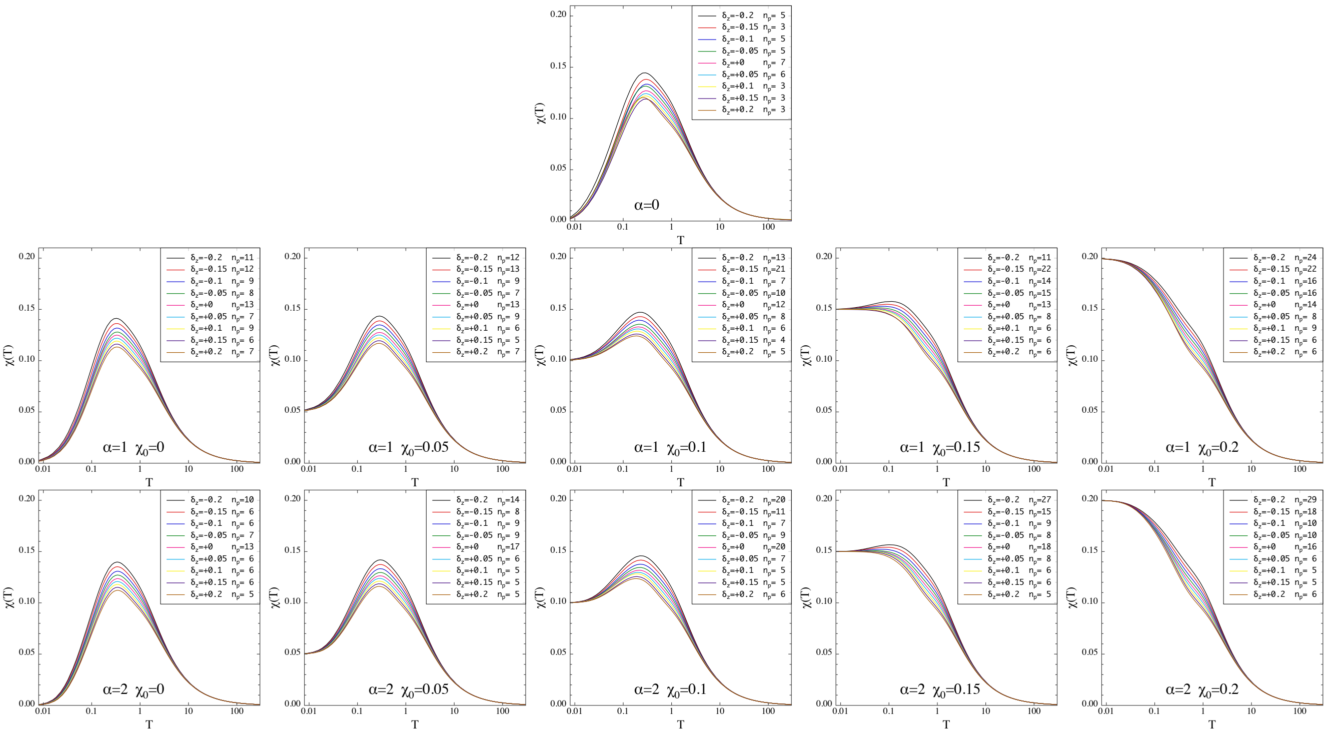


FIG. 35. Influence of an Ising anisotropy $\delta_z$ on $\chi(T)$ for $\alpha = 0$ (first raw), $\alpha = 1$ (second raw) and $\alpha = 2$ (last raw).

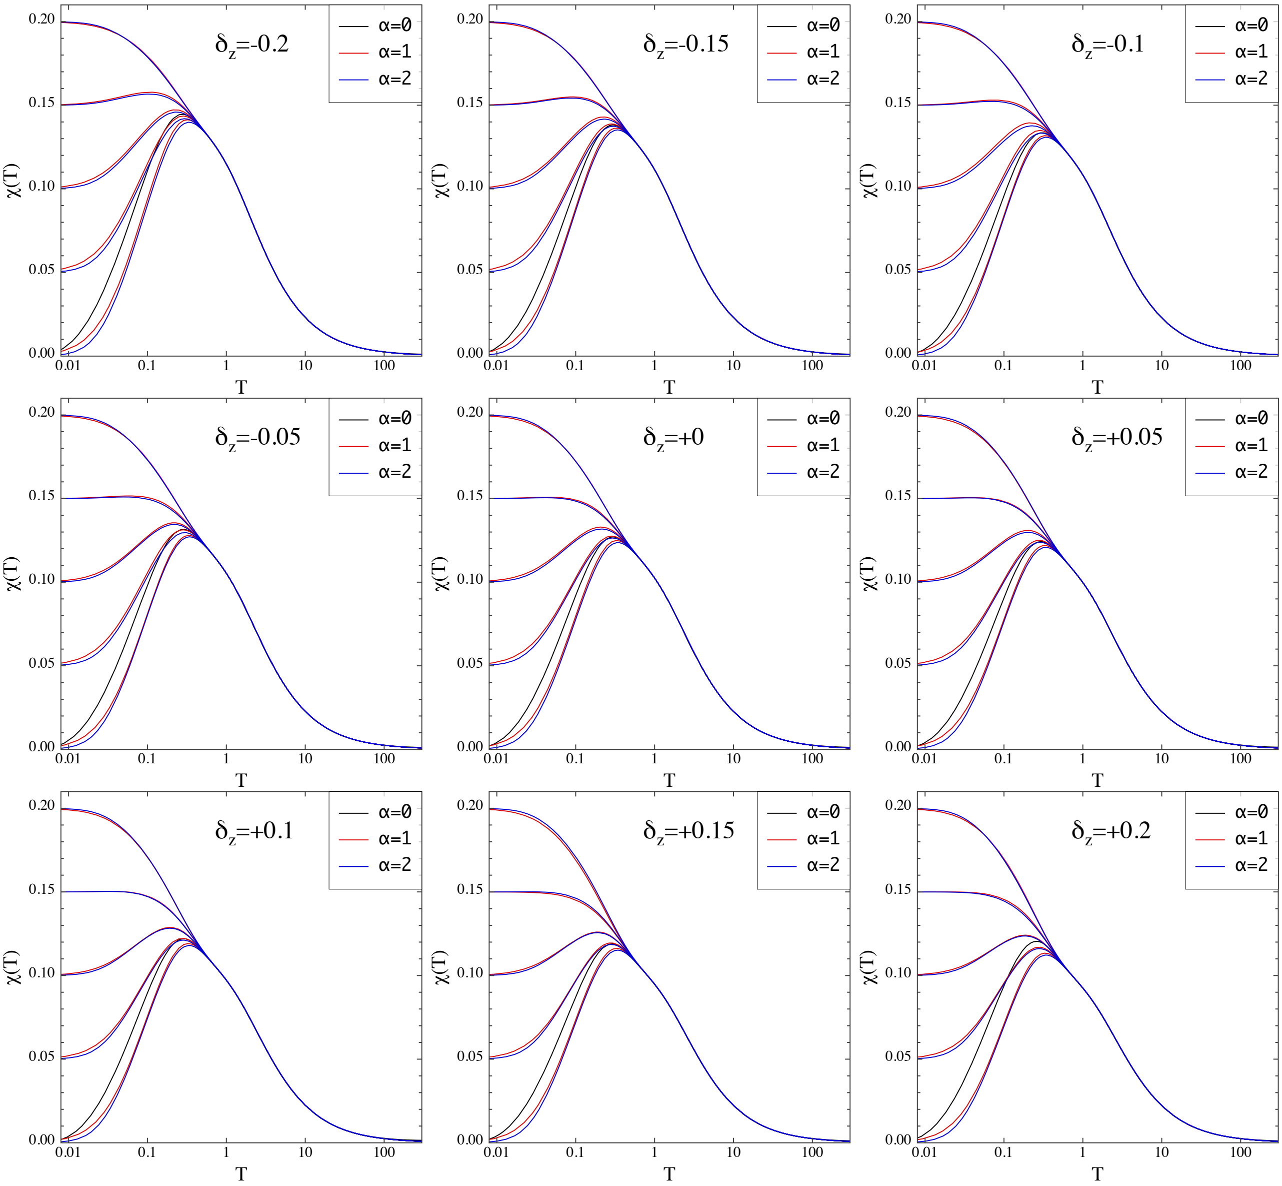


FIG. 36. Influence of an Ising anisotropy $\delta_z$ on $\chi(T)$ (same data as Fig. 35, but plotted at fixed $\delta_z$).

### E. Influence of the second neighbor interaction $J_2$

A second neighbor interaction $J_2$ is added. The HTSE of $\frac{1}{N}\ln Z$ is obtained at order 15 in $\beta$ (same data as in Sec. I F).

The ground state energy $e_0$0 varies with $J_2$. It has been adjusted on $c_V(T)$ according to the protocole of Sec.II F. Here we look at CPAs for $\beta$-orders from 13 to 15. Fig. 37 shows the effect of $J_2$ on $c_V$. The effects on $c_V(T)$ are visible in the range of temperatures between 0.1 and 1, specially for $\alpha = 2$. $e_0$ is almost constant for positive $J_2$ and decreases for negative $J_2$. For $J_2 = 0$, using these HTSE at low orders, the ground state energy is significantly lower than the one found in Sec.II F.

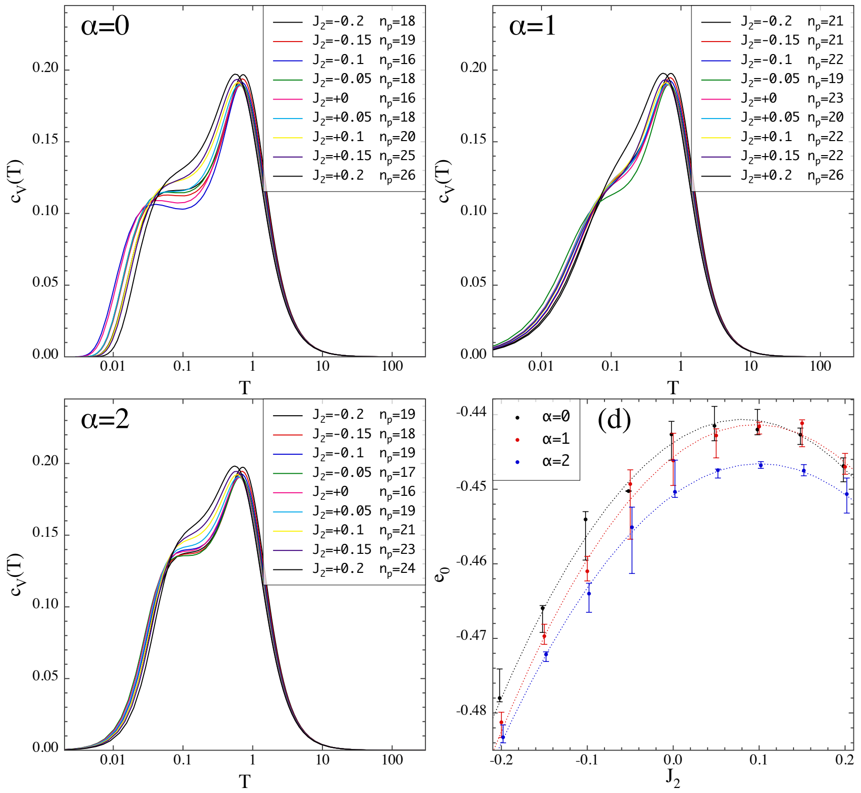


FIG. 37. Influence of a second neighbor interaction $J_2$ on $c_V(T)$ for $\alpha = 0$, 1 and 2. (d) Symbols are the ground state energy $e_0$ versus $J_2$ for $\alpha = 0$ (black), 1 (red) and 2 (blue).

Tab. XI shows the variations of the parameter $T_0$, as defined in Eqs. (27)-(30), with respect to $J_2$.

| $\delta_z$ | -0.2 | -0.15 | -0.1 | -0.05 | 0 | 0.05 | 0.1 | 0.15 | 0.2 |
|---|---|---|---|---|---|---|---|---|---|
| $\alpha = 0$ | 0.0477(17) | 0.0373(15) | 0.0488(4) | 0.05566(5) | 0.03967(21) | 0.0478(4) | 0.05686(3) | 0.0593(5) | 0.0708(6) |
| $\alpha = 1$ | 0.2692(15) | 0.3559(18) | 0.36054(28) | 0.3953(22) | 0.30715(13) | 0.3153(21) | 0.3296(20) | 0.3215(20) | 0.4192(17) |
| $\alpha = 2$ | 0.0841(3) | 0.0925(4) | 0.0916(4) | 0.0971(3) | 0.0869(4) | 0.09015(9) | 0.096657(27) | 0.10167(30) | 0.111(4) |

TABLE XI. Dependency of $T_0$ with respect to $J_2$

Figs.38-39 shows the effect of $J_2$ on the magnetic susceptibility $\chi$. The ground state energy $e_0$ is the one found for $c_V(T)$ (Fig. 37-(c)). Here, the number of CPAs is much smaller than the one found for $c_V$ and results with $n_{\text{CPA}}$ less than 5 are only qualitative.

For $J_2 = -0.2$ the $\chi(T)$ is systematically larger for $0.1 < T < 1$. Positive $J_2$ has almost no effect on $\chi(T)$.

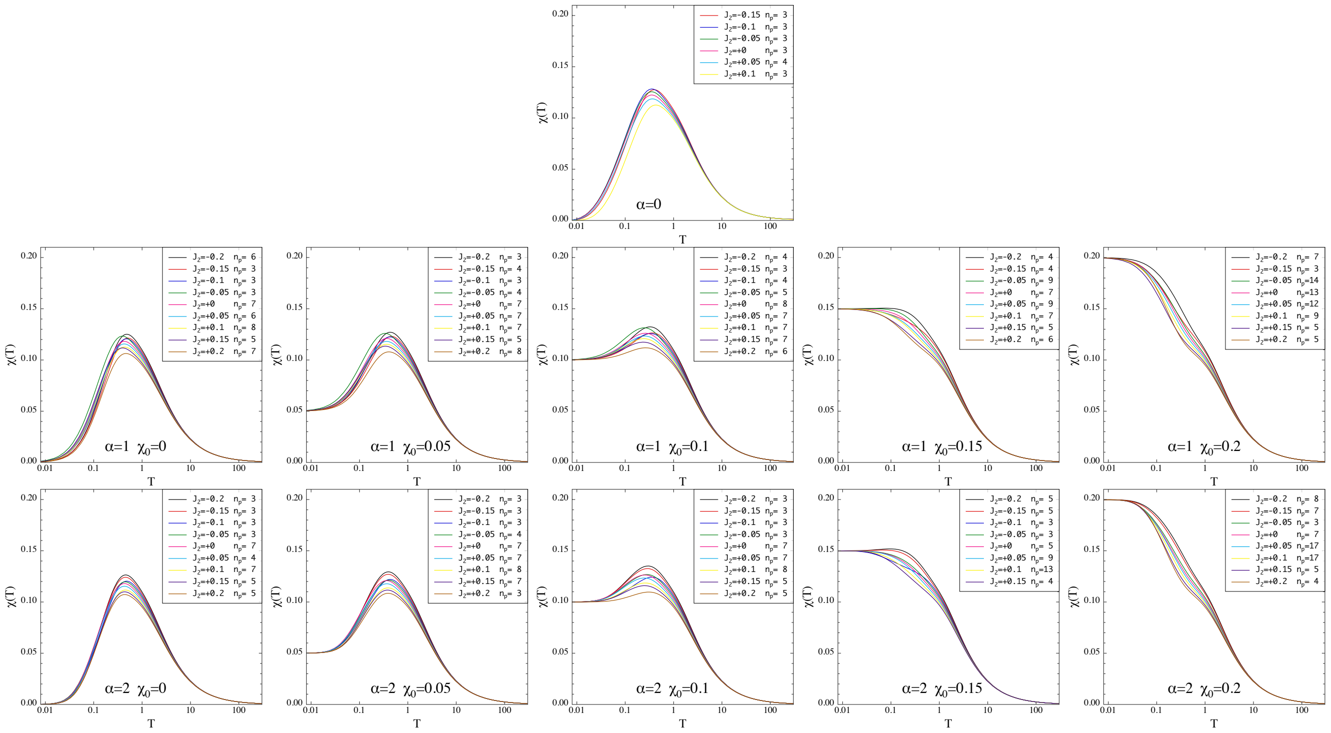


FIG. 38. Influence of a second neighbor interaction $J_2$ on $\chi(T)$ for $\alpha = 0$ (first raw), $\alpha = 1$ (second raw) and $\alpha = 2$ (last raw).

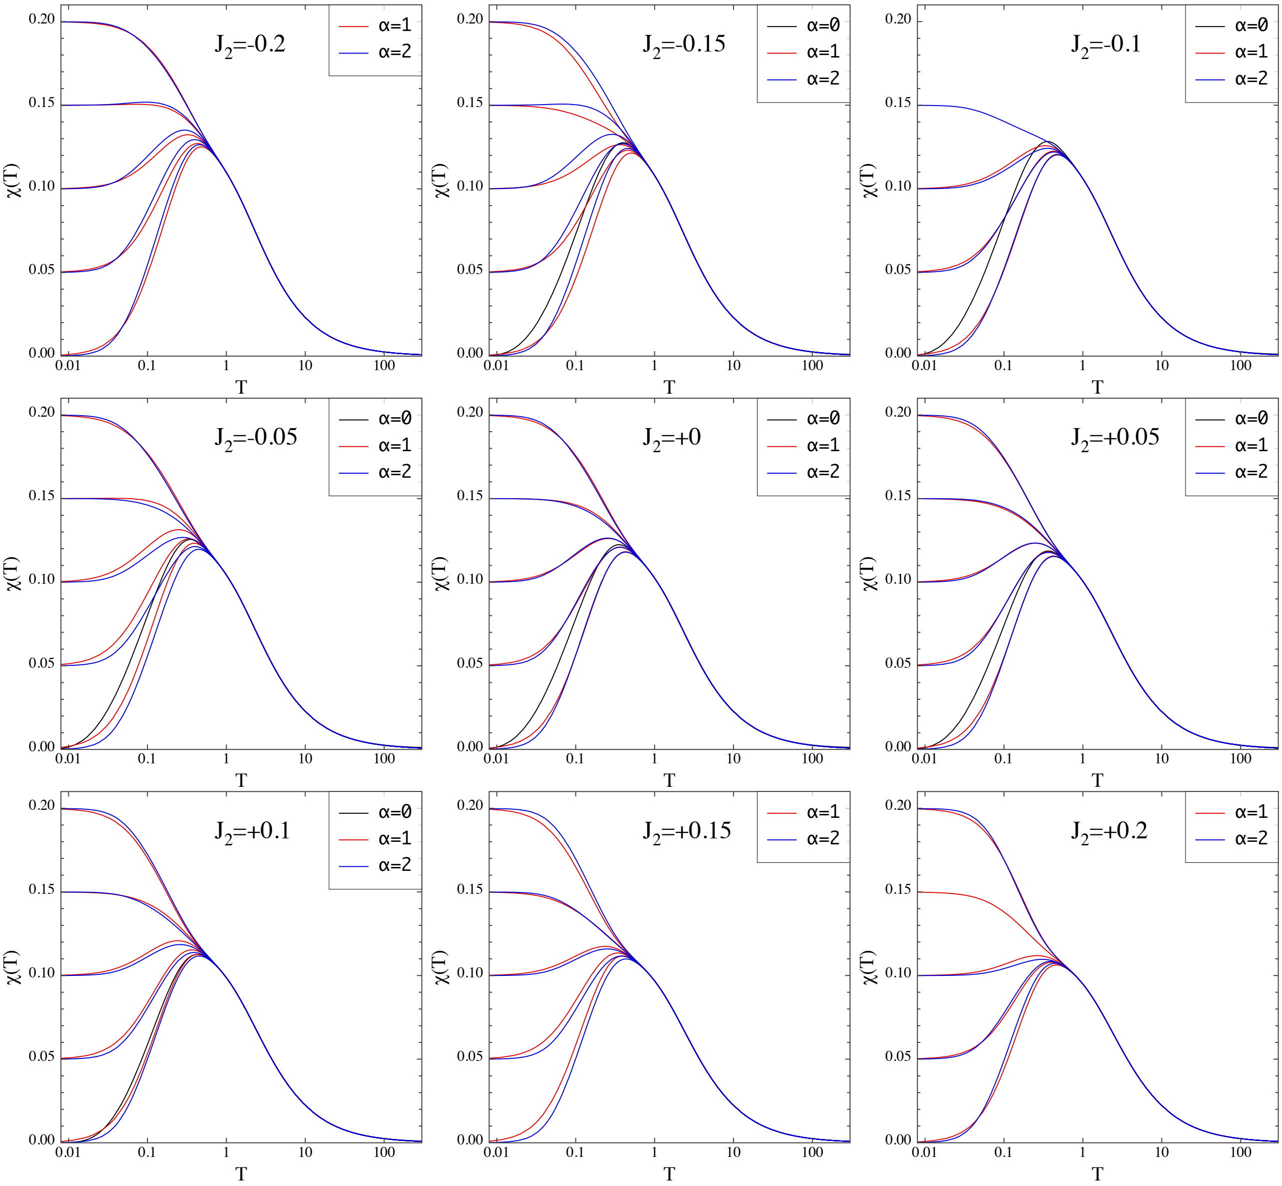


FIG. 39. Influence of a second neighbor interaction interaction $J_2$ on $\chi(T)$ (same data as Fig. 38, but plotted at fixed $J_2$).

### F. Influence of the third neighbor interaction $J_3$

An interaction $J_3$ is added. The HTSE of $\frac{1}{N}\ln Z$ is obtained at order 15 in $\beta$ (same data as in Sec. I G).

The ground state energy varies with $J_3$. It has been adjusted on $c_V(T)$ according to the protocole of Sec.II F. Here we look at CPAs for $\beta$-orders from 13 to 15. Fig. 40 shows the effect of a $J_3$ on the specific heat. $c_V(T)$ is almost unchanged in presence of this perturbation. The ground state energy $e_0$ is almost constant for positive $J_3$ and decreases for negative $J_3$ (Fig. 40-d). Quadratic fits give: $-0.4447 + 0.0605\,J_3 - 0.4324\,J_3^2$ for $\alpha = 0$, $-0.4467 + 0.06870\,J_3 - 0.3834\,J_3^2$ for $\alpha = 1$ and $-0.4511 + 0.0749\,J_3 - 0.4098\,J_3^2$ for $\alpha = 2$.

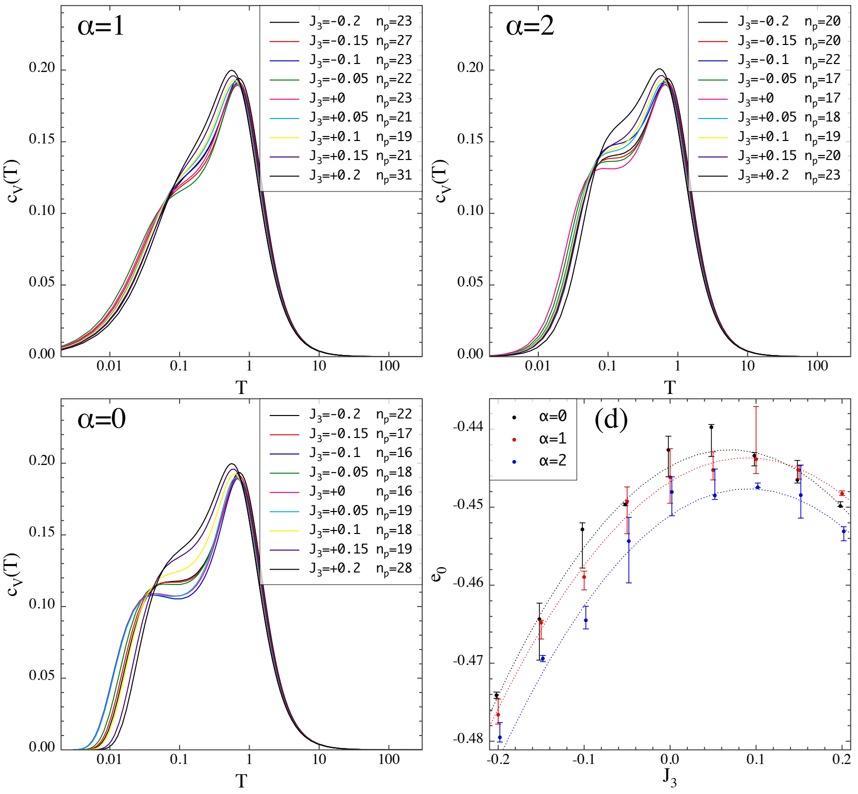


FIG. 40. (a)-(b)-(c) Influence of a third neighbor interaction $J_3$ on $c_V(T)$ for $\alpha = 1$, 2 and 0. (d) Symbols are ground state energy versus $J_3$ for $\alpha = 0$, 1 and 2. Dotted lines are quadratic fits.

Tab.XII shows the variations of the parameter $T_0$, as defined in Eqs.(27)-(30), with respect to $J_3$.

| $J_3$ | -0.2 | -0.15 | -0.1 | -0.05 | 0 | 0.05 | 0.1 | 0.15 | 0.2 |
|---|---|---|---|---|---|---|---|---|---|
| $\alpha = 0$ | 0.048413(26) | 0.0389(17) | 0.0531(3) | 0.0565(4) | 0.03967(21) | 0.0394(3) | 0.05911(6) | 0.0748(5) | 0.0848(6) |
| $\alpha = 1$ | 0.2823(15) | 0.3468(15) | 0.32183(10) | 0.3797(17) | 0.30715(13) | 0.3493(5) | 0.3555(8) | 0.3912(22) | 0.4322(18) |
| $\alpha = 2$ | 0.0842(3) | 0.1028(4) | 0.0914(3) | 0.098(4) | 0.0766(3) | 0.0923(4) | 0.0955(3) | 0.10146(6) | 0.12056(7) |

TABLE XII. Dependency of $T_0$, as defined in Eqs.(27)-(30) with respect to $J_3$.

Fig. 41-42 shows the effect of $J_3$ on the magnetic susceptibility $\chi$. The ground state energy $e_0$ is the one found for $c_V(T)$ (Fig. 40-(d)). Results with a low number of CPA must not be taken seriously, they indicate that higher order must be provided in order to get useful informations. This is at variance from the case of $c_V$ where good convergence have been found for all $J_3$. Here the number of CPAs is half that found for $c_V$ and non convergence is obtained for small negative $J_3$.

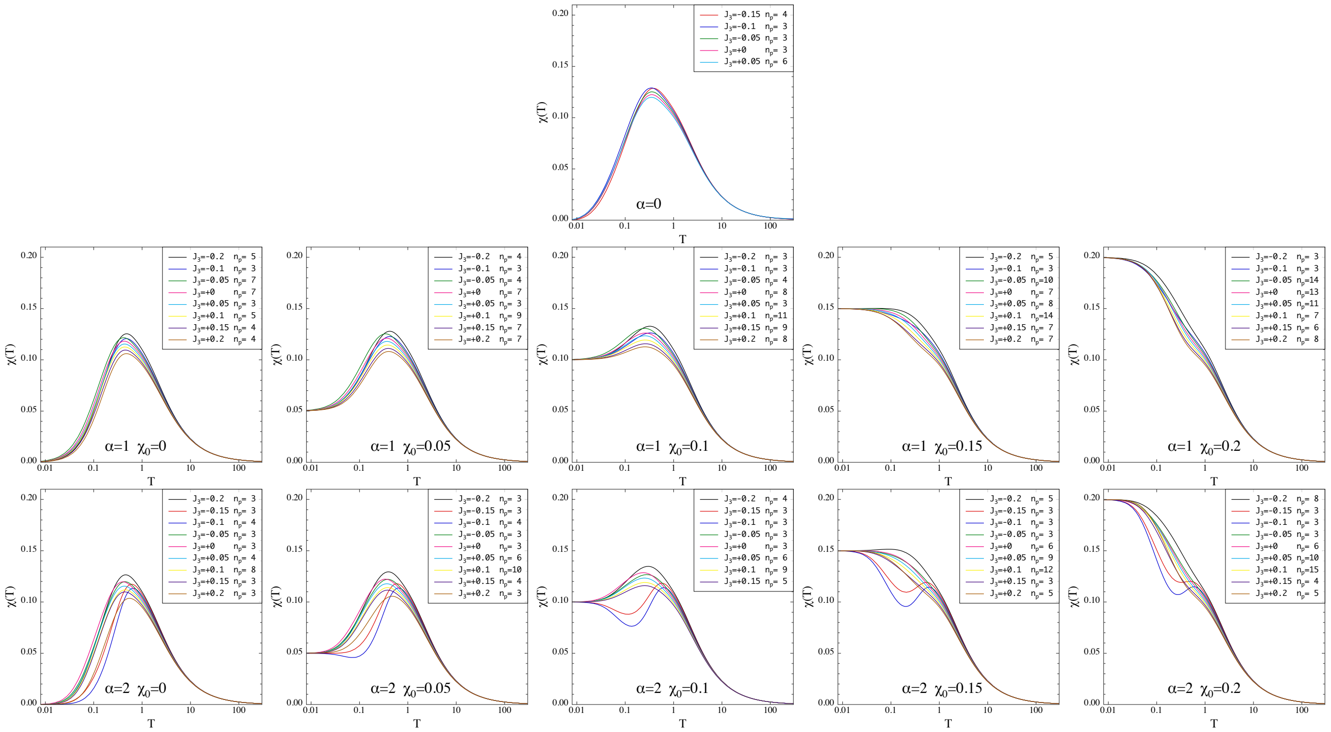


FIG. 41. Influence of a a third neighbor interaction $J_3$ on $\chi(T)$ for $\alpha = 0$ (first row), $\alpha = 1$ (second raw) and $\alpha = 2$ (last raw).

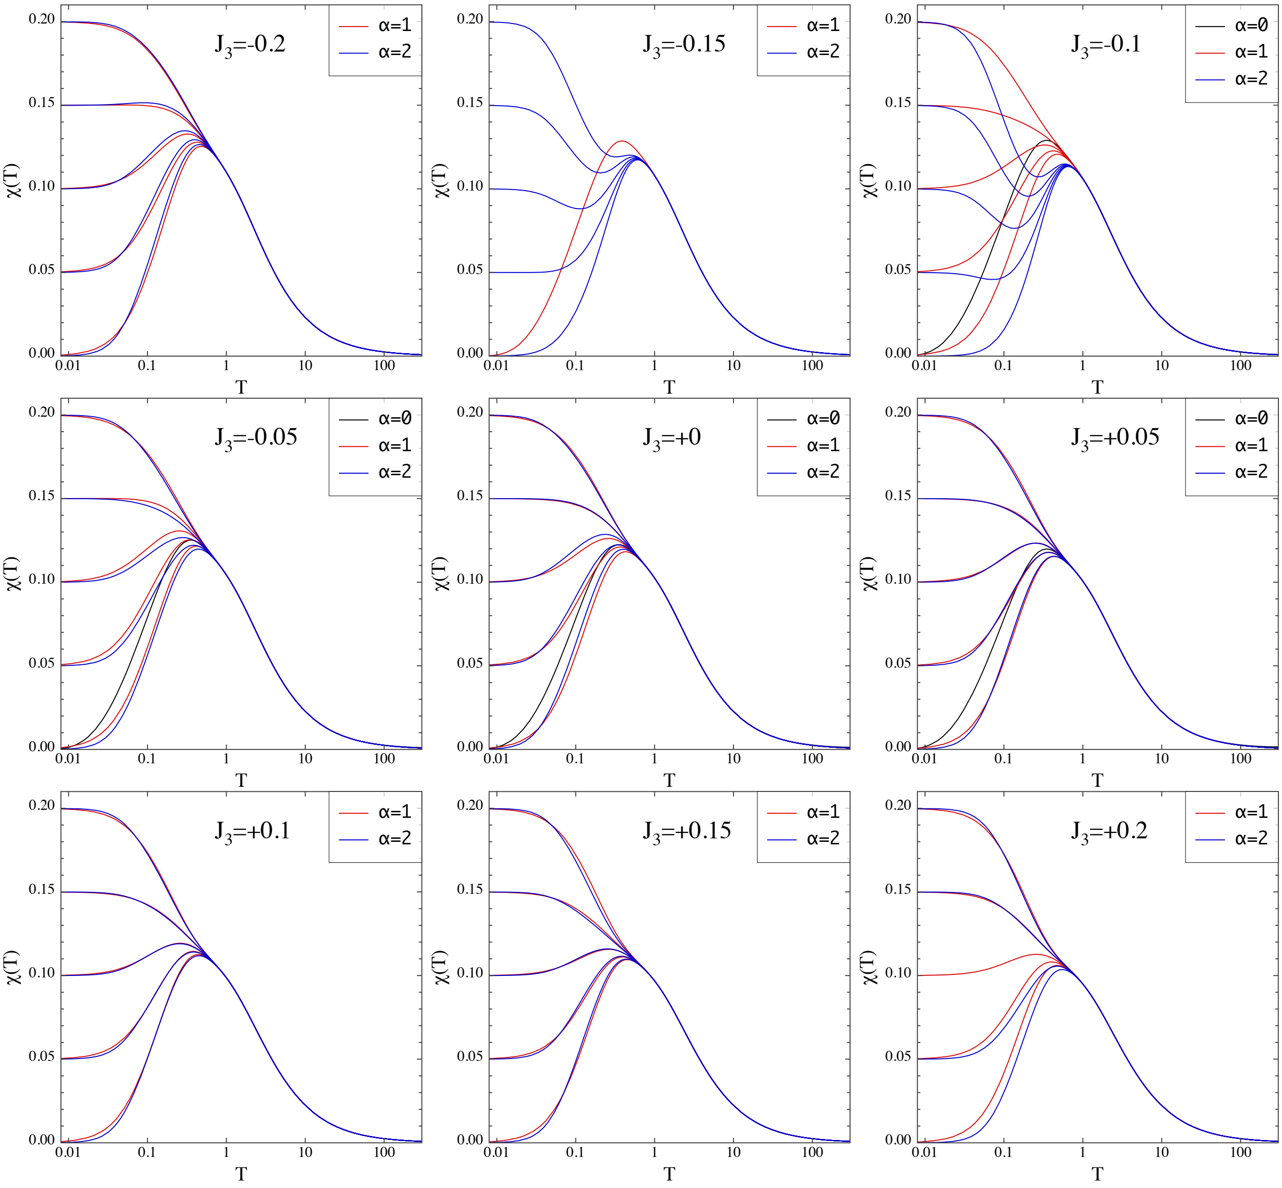


FIG. 42. Influence of a third neighbor interaction interaction $J_3$ on $\chi(T)$ (same data as Fig. 41 at fixed $J_3$).

### G. Influence of the third neighbor interaction $J_{3h}$

An interaction $J_{3h}$ is added across the hexagon. The HTSE of $\frac{1}{N}\ln Z$ is obtained at order 15 in $\beta$ (same data as in Sec. I H.

The ground state energy varies with $J_{3h}$. It has been adjusted on $c_V(T)$ according to the protocole of Sec.II F. Here we look at CPAs for $\beta$-orders from 13 to 15. Fig. 43 shows the effect of a $J_{3h}$ on the specific heat. $c_V(T)$ is almost unchanged in presence of this perturbation. The ground state energy $e_0$ is almost constant for negative $J_{3h}$ and decreases for positive perturbations (Fig. 43-d). Quadratic fits give: $-0.4448 - 0.02339\,J_{3h} - 0.21778\,J_{3h}^2$ for $\alpha = 0$, $-0.4477 - 0.02964\,J_{3h} - 0.2029\,J_{3h}^2$ for $\alpha = 1$ and $-0.4512 - 0.02899\,J_{3h} - 0.1670\,J_{3h}^2$ for $\alpha = 2$.

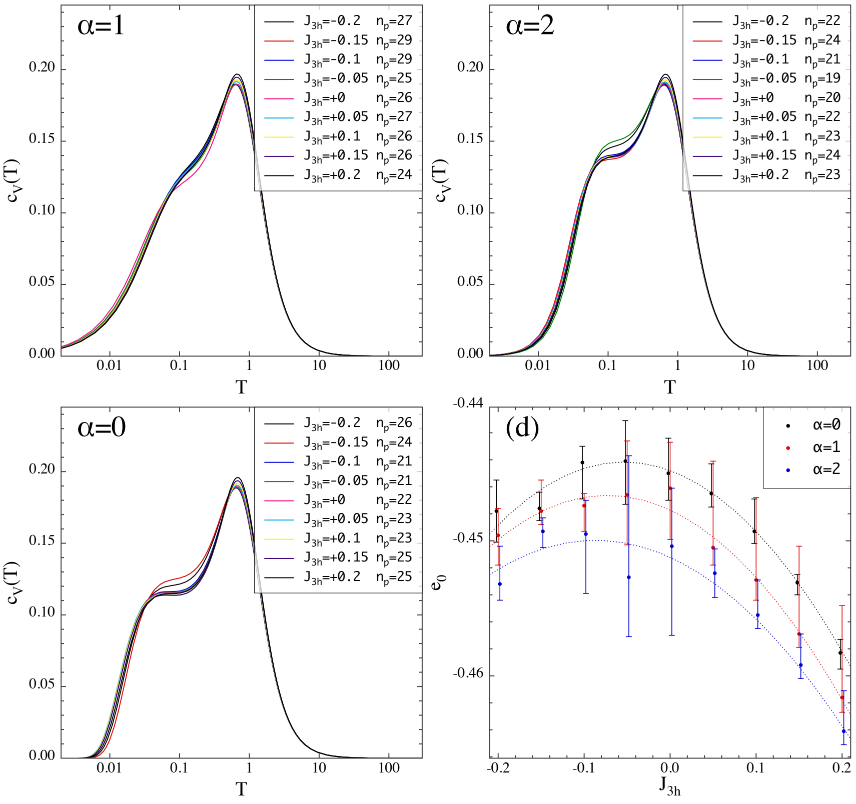


FIG. 43. (a)-(b)-(c) Influence of a third neighbor interaction across the hexagon on $c_V(T)$ for $\alpha = 1$, 2 and 0. (d) Symbols are ground state energy versus $J_{3h}$ for$\alpha = 0$, 1 and 2. Dotted lines are quadratic fits.

Tab.XIII shows the variations of the parameter $T_0$, as defined in Eqs.(27)-(30), with respect to $J_{3h}$.

| $J_{3h}$ | -0.2 | -0.15 | -0.1 | -0.05 | 0 | 0.05 | 0.1 | 0.15 | 0.2 |
|---|---|---|---|---|---|---|---|---|---|
| $\alpha = 0$ | 0.047923(15) | 0.0492(4) | 0.0602(6) | 0.0554(3) | 0.04786(7) | 0.0473(3) | 0.04803(28) | 0.04856(29) | 0.0517(4) |
| $\alpha = 1$ | 0.3336(21) | 0.3506(16) | 0.347205(21) | 0.3581(3) | 0.3083(21) | 0.3548(20) | 0.3519(14) | 0.3637(16) | 0.3729(8) |
| $\alpha = 2$ | 0.102195(26) | 0.0881(4) | 0.0846(4) | 0.0965(3) | 0.086439(25) | 0.0882(4) | 0.0901(4) | 0.0916(5) | 0.0945(5) |

TABLE XIII. Dependency of $T_0$, as defined in Eqs.(27)-(30) with respect to $J_{3h}$.

Fig. 44-45 shows the effect of $J_{3h}$ on the magnetic susceptibility $\chi$. The ground state energy $e_0$ is the one found for $c_V(T)$ (Fig. 43-(d)). Results with a low number of CPA must not be taken seriously, they indicate that higher order must be provided in order to get useful informations. This is at variance from the case of $c_V$ where good convergence have been found for all $J_{3h}$. Here the number of CPAs is half that found for $c_V$ and non convergence is obtained for small negative $J_{3h}$.

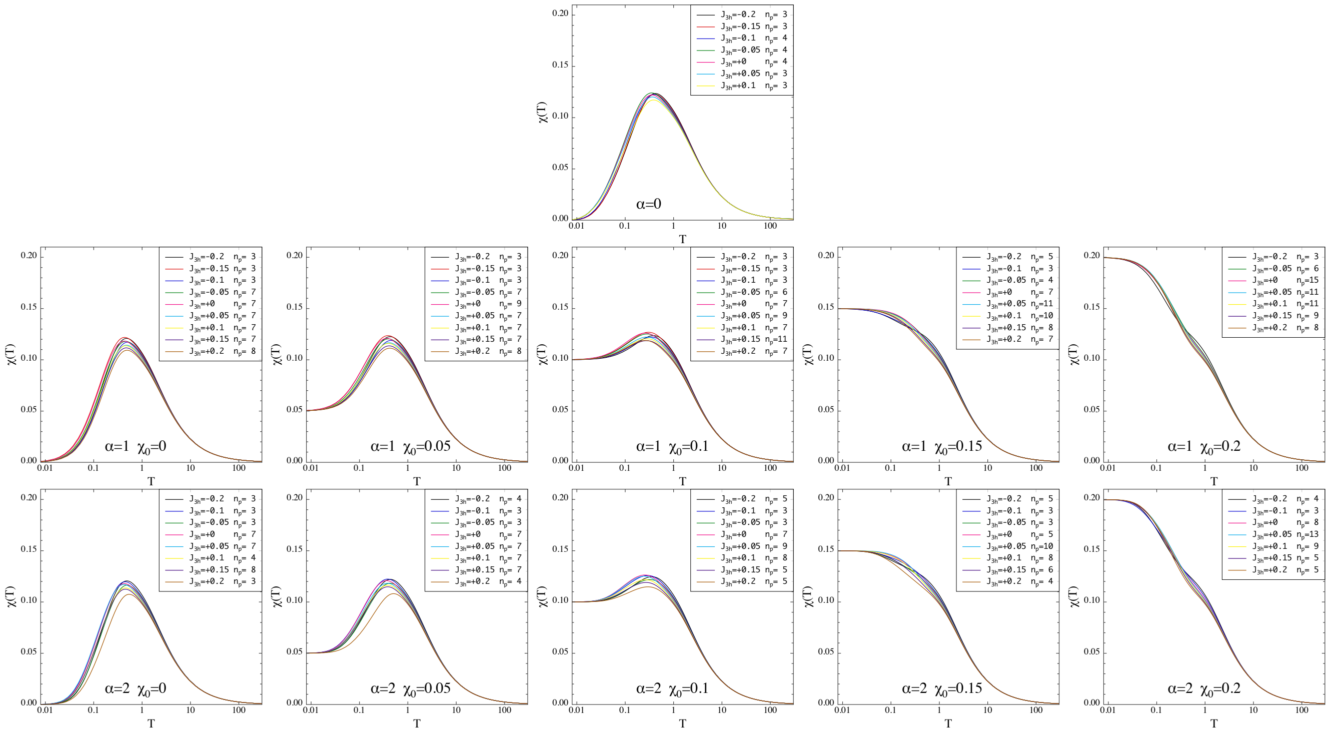


FIG. 44. Influence of a a third neighbor interaction $J_{3h}$ on $\chi(T)$ for $\alpha = 0$ (first row), $\alpha = 1$ (second raw) and $\alpha = 2$ (last raw).

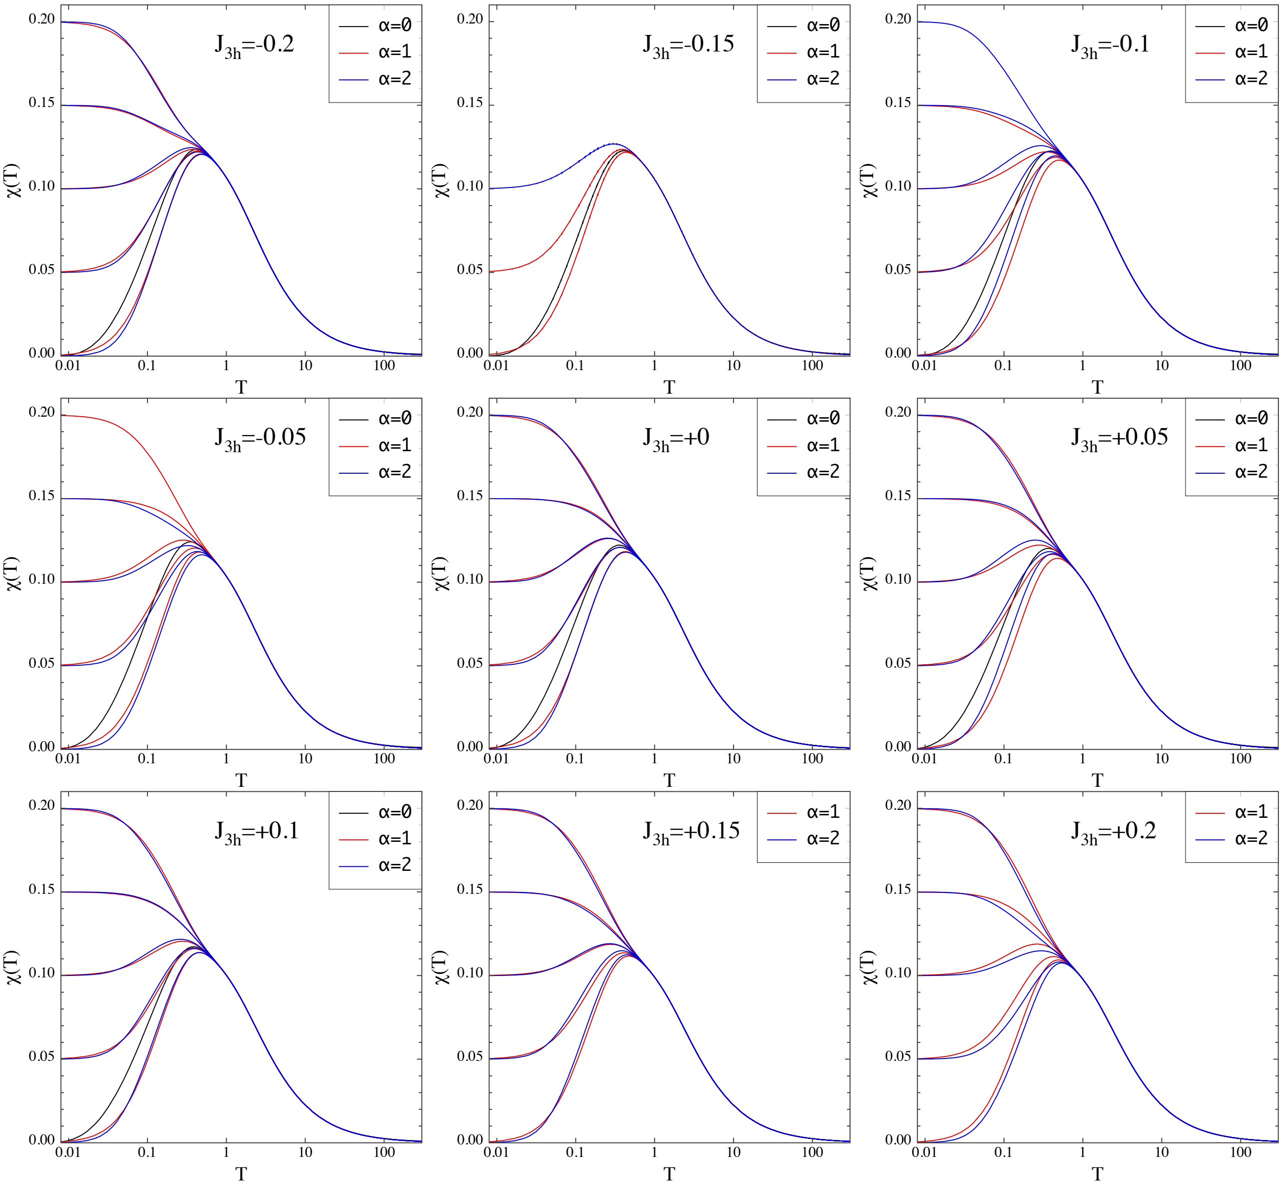


FIG. 45. Influence of a third neighbor interaction interaction $J_{3h}$ on $\chi(T)$ (same data as Fig. 44 at fixed $J_{3h}$).
